# Supplementary material for: Estimation of Multivariate Wrapped Models for Data in Torus
Source: arXiv:1811.06007 source file (2018-11-14)
Supplement: Supplementary file 1 [file torus-supplemental.pdf]

# Supplementary Material for "Estimation of Multivariate Wrapped Models for Data in Torus"

Anahita Nodehi[1], Mousa Golalizadeh[1], Mehdi Maadooliat[2], and Claudio Agostinelli[3]

[1]*Department of Statistics, Tarbiat Modares University, Tehran, Iran*
a.nodehi@modares.ac.ir, golalizadeh@modares.ac.ir
[2]*Department of Statistics, Marquette University, Milwaukee, USA*
mehdi.maadooliat@marquette.edu
[3]*Department of Mathematics, University of Trento, Trento, Italy*
claudio.agostinelli@unitn.it

# Supplementary Material

The Supplementary Material contains in Section SM–1 a discussion on the lack of equivariance properties of MLE for the Wrapped Normal models, in Section SM–2 and example based on real data set about wind direction, in Section SM–3 further results on the analysis of the RNA data set and in Section SM–4 complete results for the Monte Carlo experiments described in Section 5.

# SM–1 Equivariance in Wrapper Normal models

Let $\boldsymbol{X} \sim N_p(\boldsymbol{\mu}_X, \Sigma_X)$, $\boldsymbol{b}$ a $p$-vector and $A$ a full rank $p \times p$ matrix and let $\boldsymbol{W} = A\boldsymbol{X} + \boldsymbol{b}$ and hence $W \sim N_p(\boldsymbol{\mu}_W, \Sigma_W)$ where $\boldsymbol{\mu}_W = A\boldsymbol{\mu}_X + \boldsymbol{b}$ and $\Sigma_W = A\Sigma_X A^\top$. Define $\boldsymbol{U} = \boldsymbol{X} \mod 2\pi$ and $\boldsymbol{V} = \boldsymbol{W} \mod 2\pi$ two multivariate wrappped normal models on the $p$-torus. Hence, the density of $\boldsymbol{V}$ is equal to

$$
\begin{aligned}
f_V(\boldsymbol{v}) &= (2\pi)^{-p/2}|\Sigma_W|^{-1/2} \sum_{\boldsymbol{m}\in\mathbb{Z}^p} \exp\{(\boldsymbol{v} - \boldsymbol{\mu}_W + 2\pi\boldsymbol{m})^\top \Sigma_W^{-1}(\boldsymbol{v} - \boldsymbol{\mu}_W + 2\pi\boldsymbol{m})\} \\
&= (2\pi)^{-p/2}|A\Sigma_X A^\top|^{-1/2} \sum_{\boldsymbol{m}\in\mathbb{Z}^p} \exp\{((A\boldsymbol{x} + \boldsymbol{b}) \mod 2\pi - (A\boldsymbol{\mu}_X + \boldsymbol{b}) + 2\pi\boldsymbol{m})^\top A^{-\top}\Sigma_X^{-1}A^{-1} \\
&\times ((A\boldsymbol{x} + \boldsymbol{b}) \mod 2\pi - (A\boldsymbol{\mu}_X + \boldsymbol{b}) + 2\pi\boldsymbol{m})\} \\
&= (2\pi)^{-p/2}|A|^{-1}|\Sigma_X|^{-1/2} \sum_{\boldsymbol{m}\in\mathbb{Z}^p} \exp\{(A(\boldsymbol{x} - \boldsymbol{\mu}_X) + 2\pi\boldsymbol{m})^\top A^{-\top}\Sigma_X^{-1}A^{-1}(A(\boldsymbol{x} - \boldsymbol{\mu}_X) + 2\pi\boldsymbol{m})\} \\
&= (2\pi)^{-p/2}|A|^{-1}|\Sigma_X|^{-1/2} \sum_{\boldsymbol{m}\in\mathbb{Z}^p} \exp\{(\boldsymbol{x} - \boldsymbol{\mu}_X + 2\pi A^{-1}\boldsymbol{m})^\top \Sigma_X^{-1}(\boldsymbol{x} - \boldsymbol{\mu}_X + 2\pi A^{-1}\boldsymbol{m})\} \\
&= |A|^{-1} f_{U^*}(\boldsymbol{u}^*)
\end{aligned}
$$

where $\boldsymbol{U}^* = \boldsymbol{X} \mod (2\pi A^{-1}\boldsymbol{j})$ and $\boldsymbol{j}$ is a $p$-vector of ones. As a consequence we have that

$$
L(\mu_W, \Sigma_W|\boldsymbol{v}_1, \cdots, \boldsymbol{v}_n) = \prod_{i=1}^n f_V(\boldsymbol{v}_i) \propto \prod_{i=1}^n f_{U^*}(\boldsymbol{u}_i^*) \not\propto \prod_{i=1}^n f_U(\boldsymbol{u}_i) = L(\mu_X, \Sigma_X|\boldsymbol{u}_1, \cdots, \boldsymbol{u}_n)
$$

and the MLE estimates can not be affine equivariant for this model.

## SM–2 Wind direction: univariate case

In a place named "Col de la Roa" in the Italian Alps there is a meteorological station that records via data-logger several parameters. Measures are made every 15 minutes, in this dataset we report the wind direction recorded every day from January 29, 2001 to March 31, 2001 from 3.00 a.m. to 4.00 a.m. included. Which means 5 observations every day for a total of 310 measures (for more information, one can visit `intra.tesaf.unipd.it/Sanvito`). This dataset is also available in the `circular` package. Here we use EM, CEM, direct optimization of the loglikelihood using `optim` R function (optim) and R function `mle.wrappednormal` from `circular` package (MLE) to estimate the parameters. To evaluate their performance we report the angular separation (AS) and the mean square error (MSE) estimated using 5000 bootstrap replications.

Table SM–1: Wind data set. Estimates and associated bootstrap measure of variability.

| Methods | $\hat{\mu}$ | $AS(\hat{\mu})$ | $\hat{\sigma}$ | $MSE(\hat{\sigma})$ |
|---|---|---|---|---|
| EM | 0.4274 | 0.0020 | 1.0050 | 0.0029 |
| CEM | 0.4924 | 0.0035 | 0.9981 | 0.0027 |
| optim | 0.4273 | 0.0020 | 1.0049 | 0.0031 |
| MLE | 0.4274 | 0.0021 | 1.0050 | 0.0030 |

In table SM–1, we report the results. All the methods performs equally well, we just notice that CEM is the one behaving more differently from the others.

## SM–3 RNA data set: 7-torus

In Tables SM–2 and SM–3, we report the mean estimation for all 23 clusters based on the EM and CEM algorithms. In addition, Figures SM–1 – SM–6 show each correlation by an ellipse in each clusters with both the EM and CEM.

| Cluster # | # points | $\alpha$ | $\beta$ | $\gamma$ | $\delta$ | $\epsilon$ | $\zeta$ | $\chi$ |
|---|---|---|---|---|---|---|---|---|
| 1 | 4917 | 294.51 | 174.32 | 53.19 | 81.69 | 209.43 | 289.06 | 198.49 |
| 2 | 477 | 147.87 | 201.64 | 176.65 | 83.95 | 226.05 | 283.47 | 184.08 |
| 3 | 232 | 293.02 | 172.99 | 56.25 | 83.96 | 215.97 | 274.98 | 206.45 |
| 4 | 211 | 180.71 | 169.80 | 55.33 | 84.15 | 217.79 | 289.43 | 193.96 |
| 5 | 140 | 294.18 | 172.25 | 54.90 | 84.30 | 209.35 | 69.46 | 208.24 |
| 6 | 139 | 76.10 | 166.62 | 54.35 | 84.81 | 217.13 | 278.62 | 190.86 |
| 7 | 139 | 301.69 | 184.05 | 56.40 | 142.32 | 231.30 | 173.97 | 249.90 |
| 8 | 138 | 295.20 | 175.25 | 53.05 | 83.11 | 226.93 | 204.82 | 205.91 |
| 9 | 128 | 296.46 | 184.39 | 50.28 | 144.61 | 259.61 | 97.66 | 238.22 |
| 10 | 122 | 221.60 | 122.08 | 159.52 | 84.57 | 223.97 | 286.50 | 182.48 |
| 11 | 85 | 298.45 | 324.62 | 56.75 | 142.77 | 112.56 | 282.31 | 243.48 |
| 12 | 84 | 149.85 | 215.57 | 171.33 | 90.85 | 247.94 | 227.26 | 194.70 |
| 13 | 79 | 83.66 | 188.06 | 183.44 | 84.66 | 118.97 | 290.87 | 298.57 |
| 14 | 72 | 75.80 | 190.03 | 57.96 | 146.31 | 260.59 | 278.93 | 240.86 |
| 15 | 60 | 163.88 | 164.96 | 53.56 | 146.89 | 259.73 | 124.57 | 226.98 |
| 16 | 60 | 260.44 | 9.37 | 0.24 | 102.52 | 47.76 | 248.09 | 359.36 |
| 17 | 59 | 66.27 | 165.89 | 52.84 | 123.51 | 231.12 | 98.14 | 230.68 |
| 18 | 54 | 53.53 | 184.76 | 287.72 | 93.89 | 206.73 | 302.20 | 200.95 |
| 19 | 52 | 290.98 | 176.79 | 56.04 | 93.08 | 27.33 | 113.56 | 219.95 |
| 20 | 46 | 320.36 | 208.45 | 62.14 | 102.25 | 296.90 | 188.88 | 286.98 |
| 21 | 35 | 176.22 | 163.80 | 53.25 | 141.37 | 263.44 | 277.16 | 234.71 |
| 22 | 33 | 266.28 | 233.51 | 282.95 | 87.91 | 203.45 | 293.86 | 194.22 |
| 23 | 28 | 293.77 | 194.83 | 51.96 | 90.17 | 79.14 | 284.70 | 235.88 |

Table SM–2: Estimated mean of each of the 23 clusters by EM algorithm.

| Cluster # | # points | $\alpha$ | $\beta$ | $\gamma$ | $\delta$ | $\epsilon$ | $\zeta$ | $\chi$ |
|---|---|---|---|---|---|---|---|---|
| 1 | 4917 | 294.51 | 174.32 | 53.19 | 81.69 | 209.43 | 289.06 | 198.49 |
| 2 | 477 | 147.87 | 201.64 | 176.65 | 83.95 | 226.05 | 283.47 | 184.08 |
| 3 | 232 | 293.02 | 172.99 | 56.25 | 83.96 | 215.97 | 274.98 | 206.45 |
| 4 | 211 | 180.71 | 169.80 | 55.33 | 84.15 | 217.79 | 289.43 | 193.96 |
| 5 | 140 | 294.18 | 172.25 | 54.90 | 84.30 | 209.35 | 69.46 | 208.24 |
| 6 | 139 | 76.10 | 166.62 | 54.35 | 84.81 | 217.13 | 278.62 | 190.86 |
| 7 | 139 | 301.69 | 184.05 | 56.40 | 142.32 | 231.30 | 173.97 | 249.90 |
| 8 | 138 | 295.20 | 175.25 | 53.05 | 83.11 | 226.93 | 204.82 | 205.91 |
| 9 | 128 | 296.46 | 184.39 | 50.28 | 144.61 | 259.61 | 97.66 | 238.22 |
| 10 | 122 | 221.60 | 122.08 | 159.52 | 84.57 | 223.97 | 286.50 | 182.48 |
| 11 | 85 | 298.45 | 180.42 | 56.75 | 142.77 | 256.77 | 282.31 | 243.48 |
| 12 | 84 | 149.85 | 215.57 | 171.33 | 90.85 | 247.94 | 226.92 | 194.70 |
| 13 | 79 | 83.66 | 188.06 | 183.44 | 84.66 | 220.79 | 290.87 | 196.75 |
| 14 | 72 | 75.80 | 190.03 | 57.96 | 146.31 | 260.59 | 278.93 | 240.86 |
| 15 | 60 | 163.88 | 164.96 | 53.56 | 146.89 | 259.73 | 124.57 | 226.98 |
| 16 | 60 | 272.41 | 15.36 | 354.25 | 102.52 | 53.74 | 248.09 | 353.37 |
| 17 | 59 | 66.27 | 165.89 | 52.84 | 123.51 | 231.12 | 98.14 | 230.68 |
| 18 | 54 | 53.53 | 184.76 | 287.72 | 93.89 | 206.73 | 302.20 | 200.95 |
| 19 | 52 | 290.98 | 176.79 | 56.04 | 93.08 | 27.33 | 113.56 | 219.95 |
| 20 | 46 | 337.29 | 208.45 | 62.14 | 102.25 | 313.83 | 171.95 | 303.91 |
| 21 | 35 | 176.22 | 163.80 | 53.25 | 141.37 | 263.44 | 277.16 | 234.71 |
| 22 | 33 | 266.28 | 233.51 | 282.95 | 87.91 | 203.45 | 293.86 | 194.22 |
| 23 | 28 | 293.77 | 194.83 | 51.96 | 90.17 | 79.14 | 284.70 | 235.88 |

Table SM–3: Estimated mean of each of the 23 clusters by CEM algorithm.

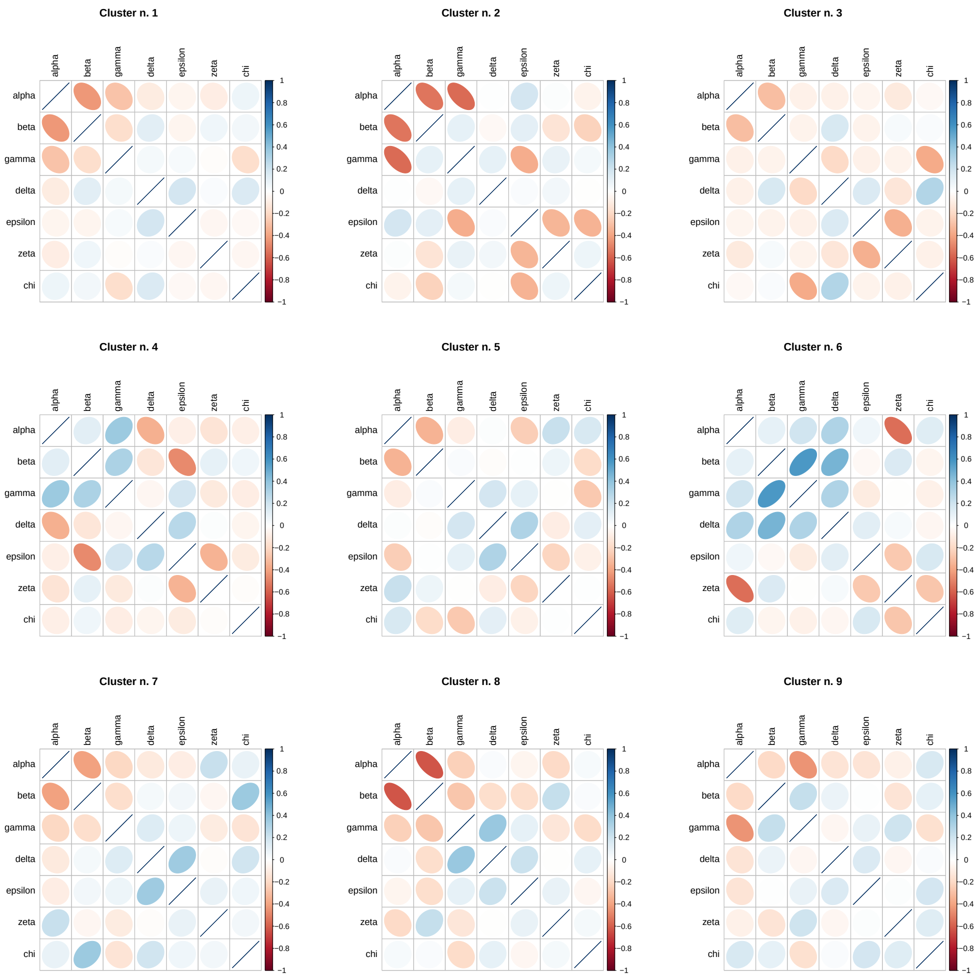


Figure SM–1: RNA data set. EM Estimated correlation matrix for clusters 1-9.

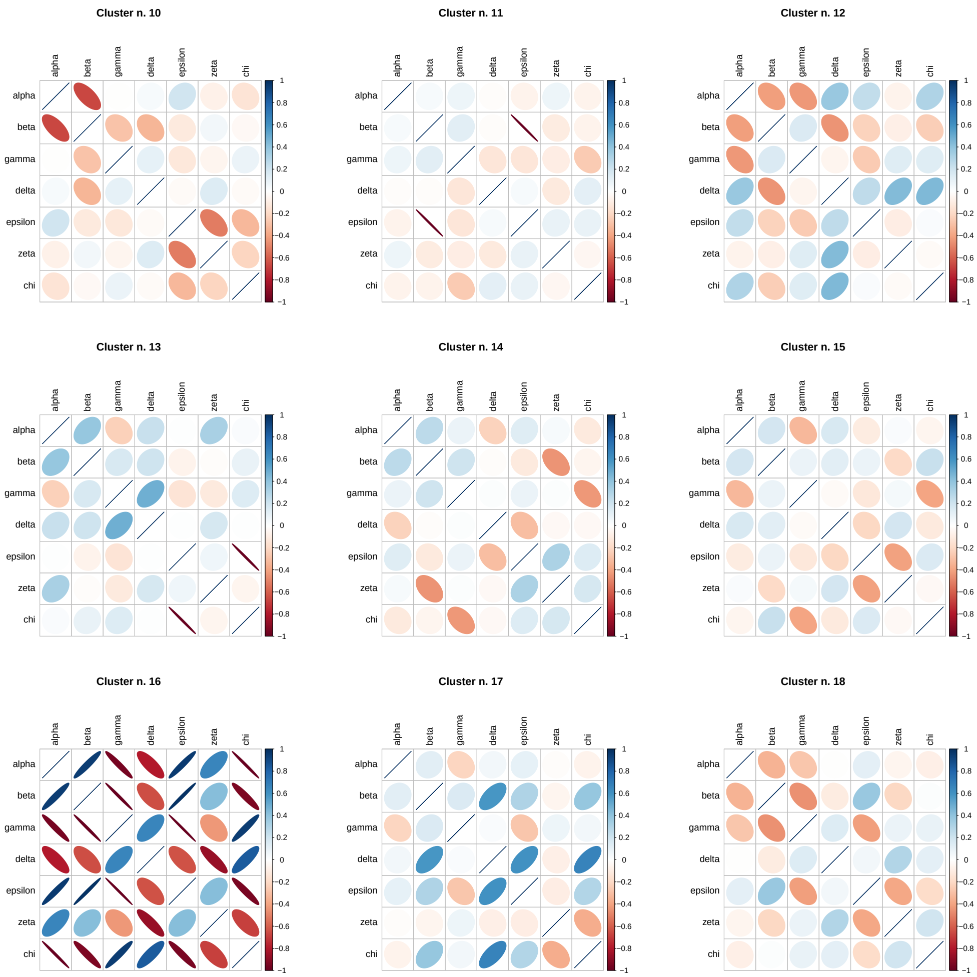


Figure SM–2: RNA data set. EM Estimated correlation matrix for clusters 10-18.

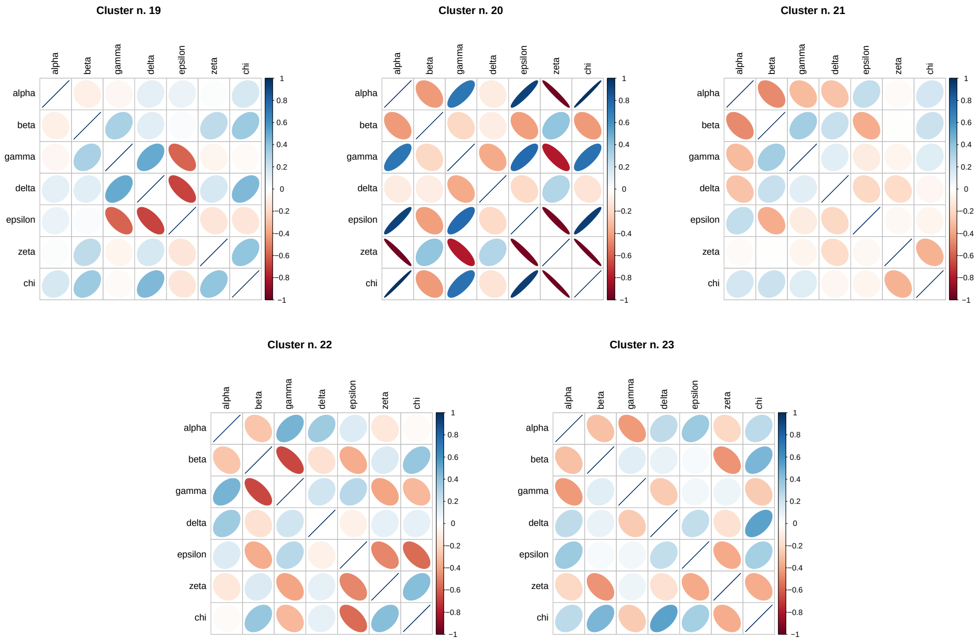


Figure SM–3: RNA data set. EM Estimated correlation matrix for clusters 19-23.

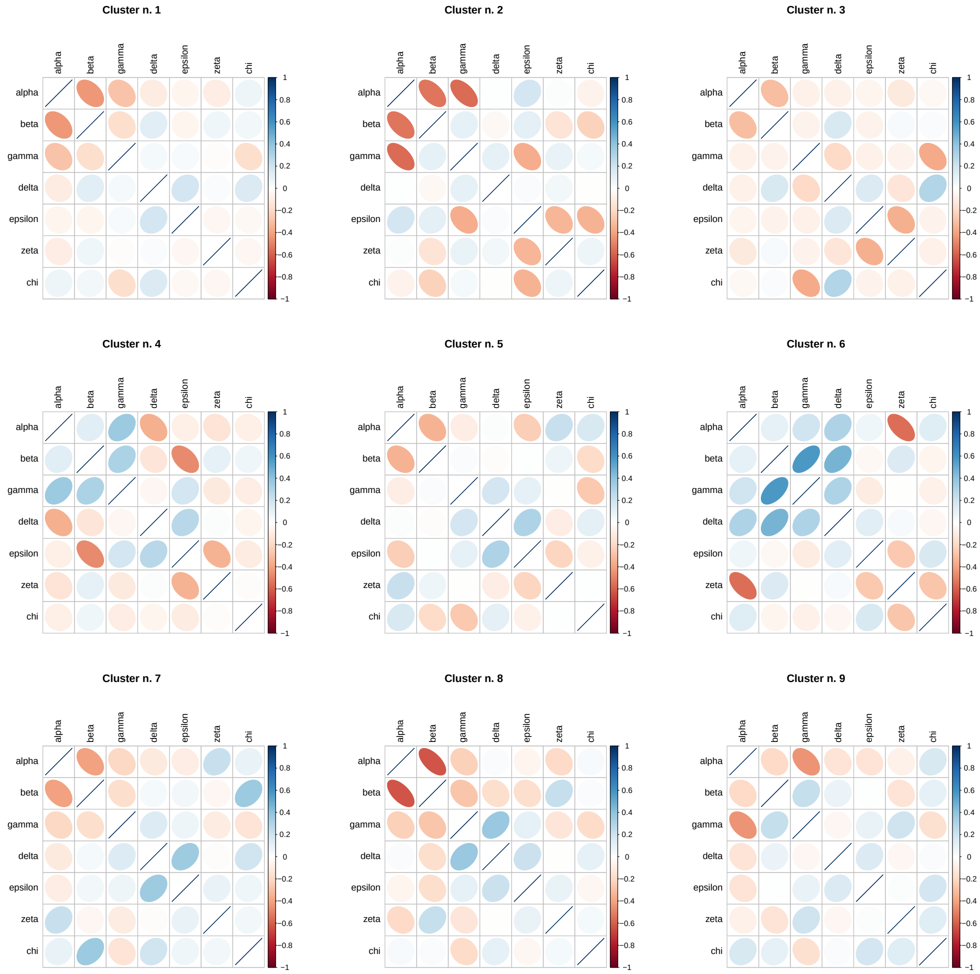


Figure SM–4: RNA data set. CEM Estimated correlation matrix for clusters 1-9.

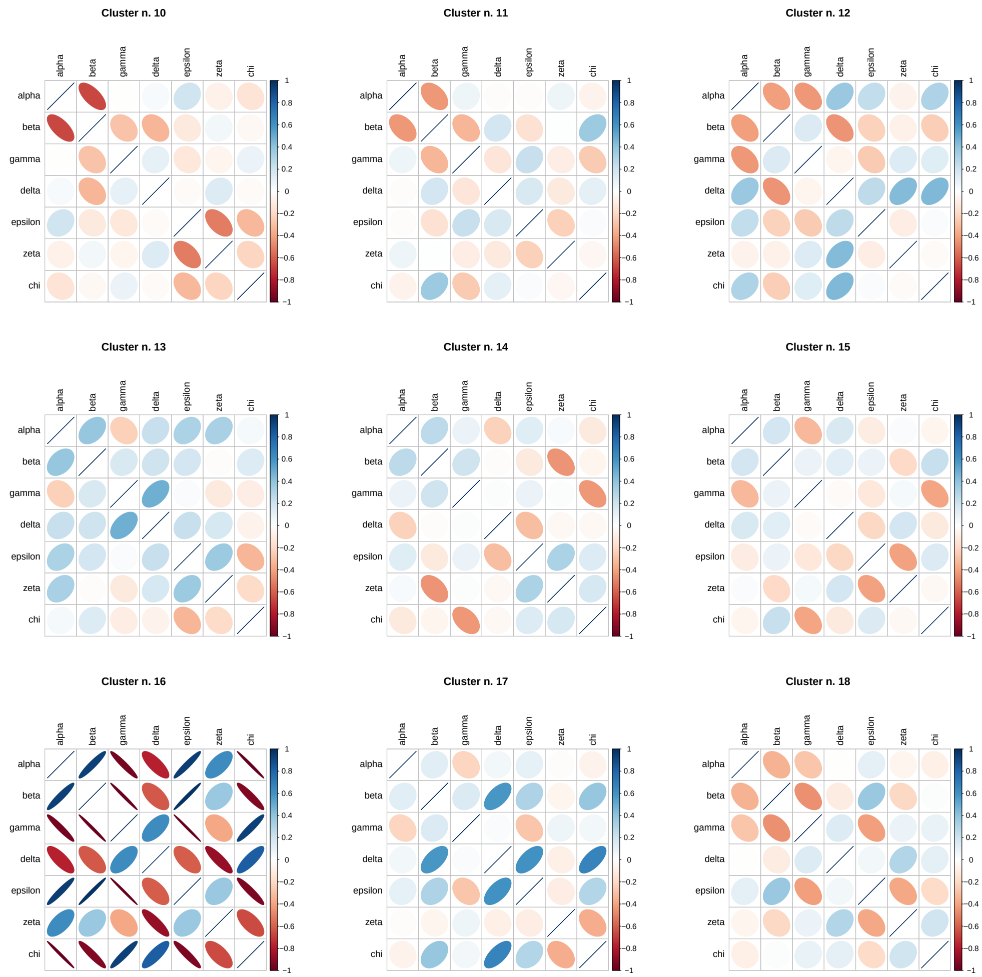


Figure SM–5: RNA data set. CEM Estimated correlation matrix for clusters 10-18.

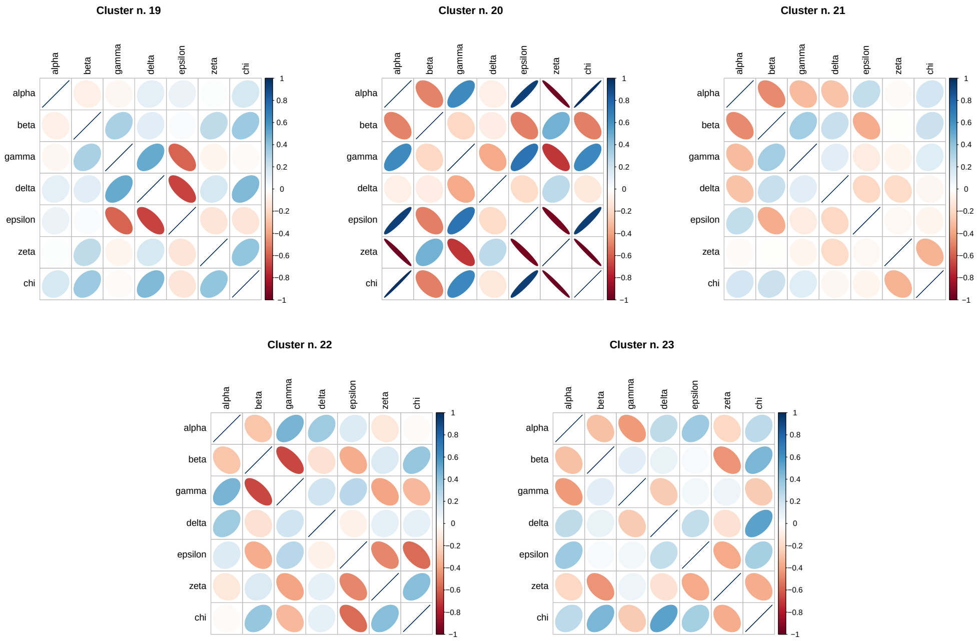


Figure SM–6: RNA data set. CEM Estimated correlation matrix for clusters 19-23.

# SM–4 Monte Carlo experiments

Complete results of the Monte Carlo experiments illustrated in Section 5 of the main paper are reported in the next subsections.

## SM–4.1 $p = 1$

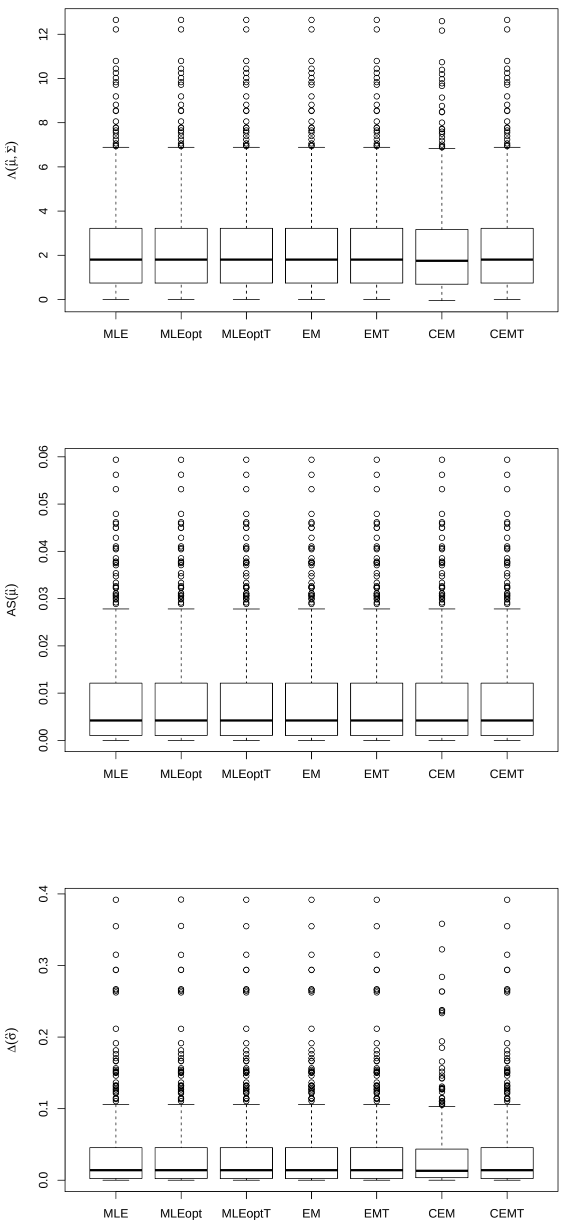


Figure SM–7: Performance of the estimators in the univariate case $p = 1$, sample size $n = 10$, $\sigma = \pi/8$.

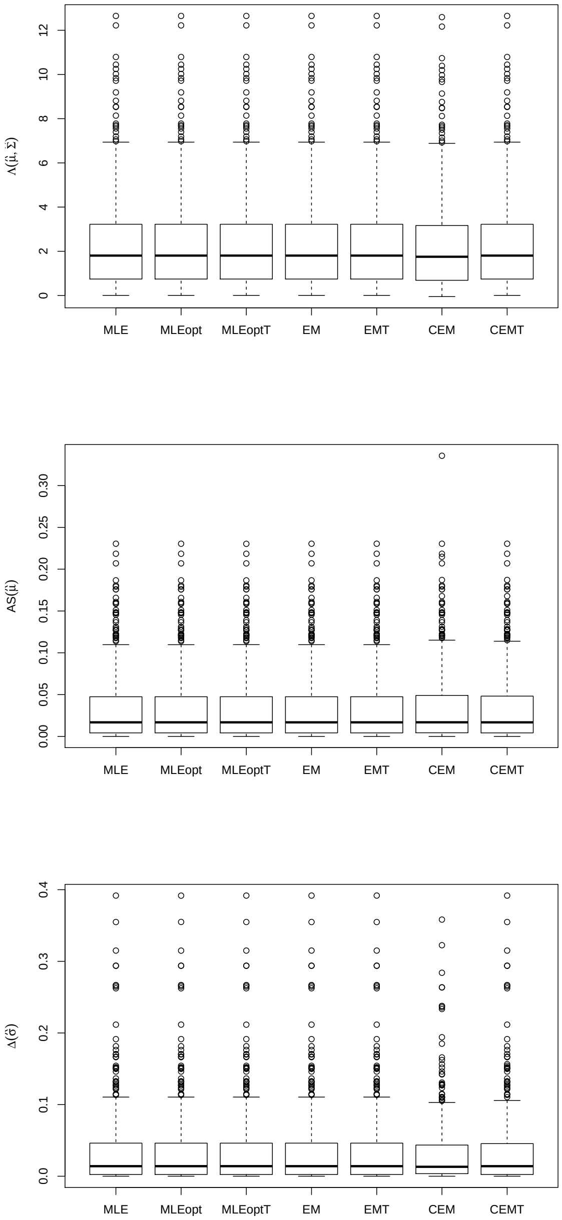


Figure SM–8: Performance of the estimators in the univariate case $p = 1$, sample size $n = 10$, $\sigma = \pi/4$.

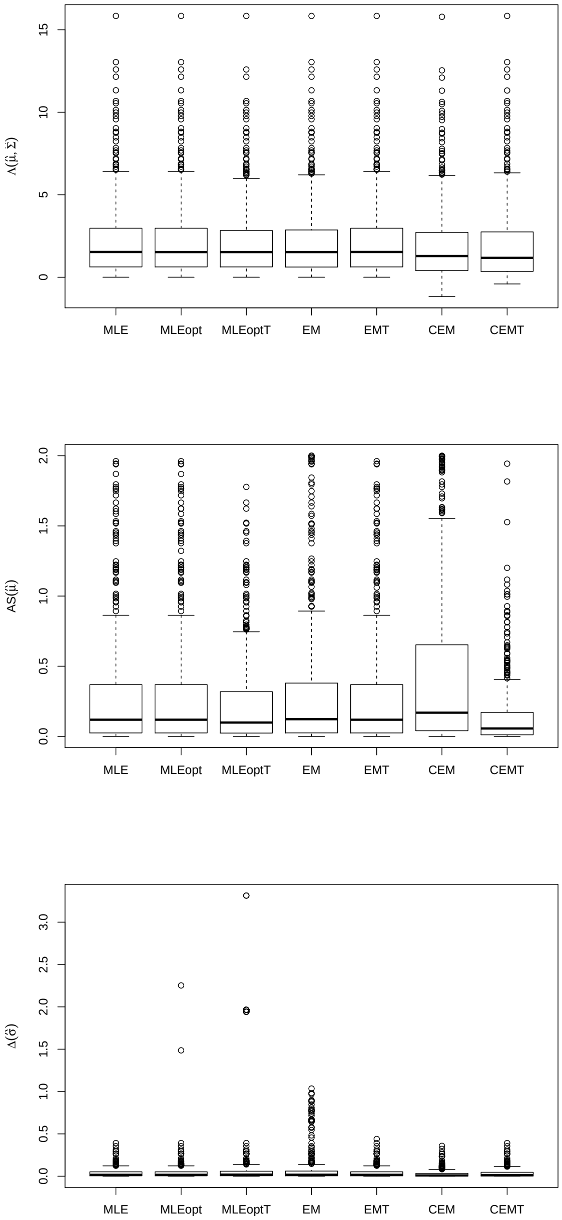


Figure SM–9: Performance of the estimators in the univariate case $p = 1$, sample size $n = 10$, $\sigma = \pi/2$.

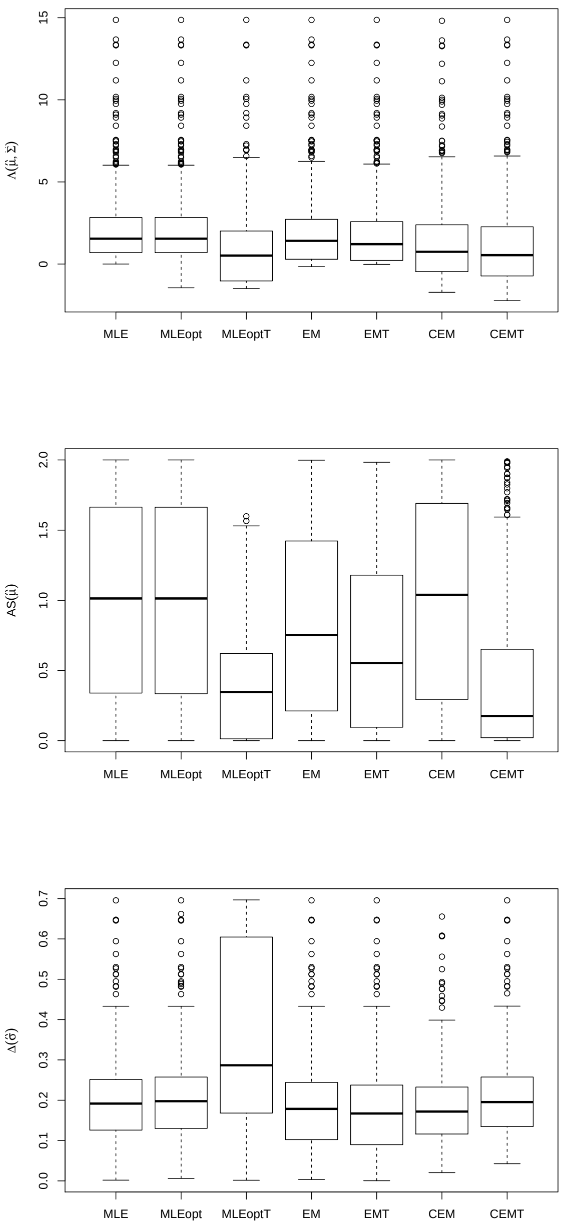


Figure SM–10: Performance of the estimators in the univariate case $p = 1$, sample size $n = 10$, $\sigma = \pi$.

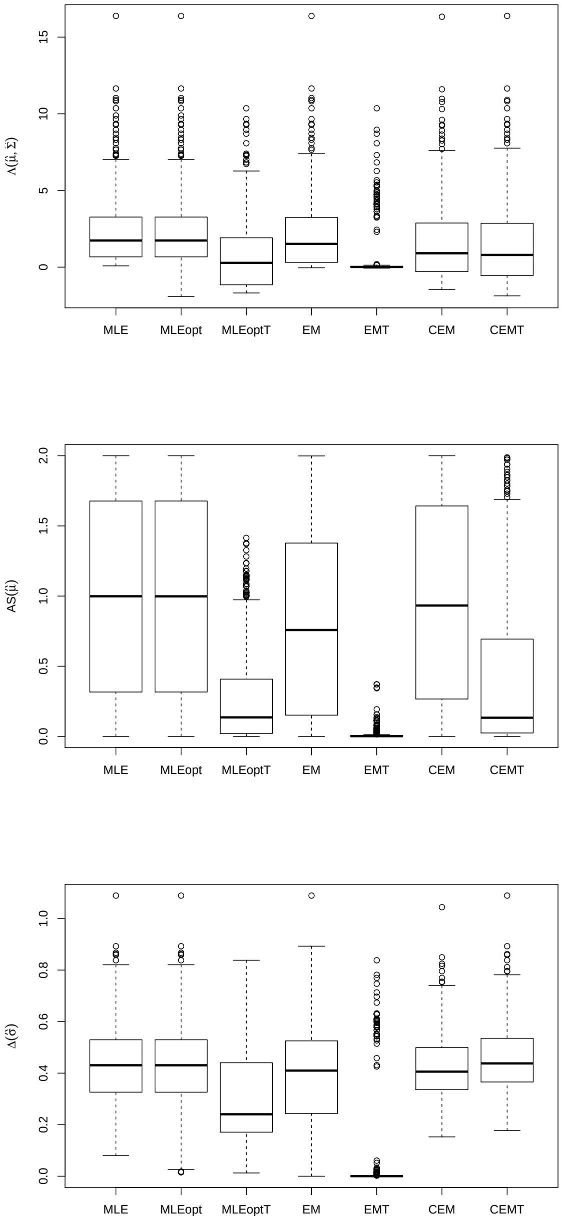


Figure SM–11: Performance of the estimators in the univariate case $p = 1$, sample size $n = 10$, $\sigma = 3\pi/2$.

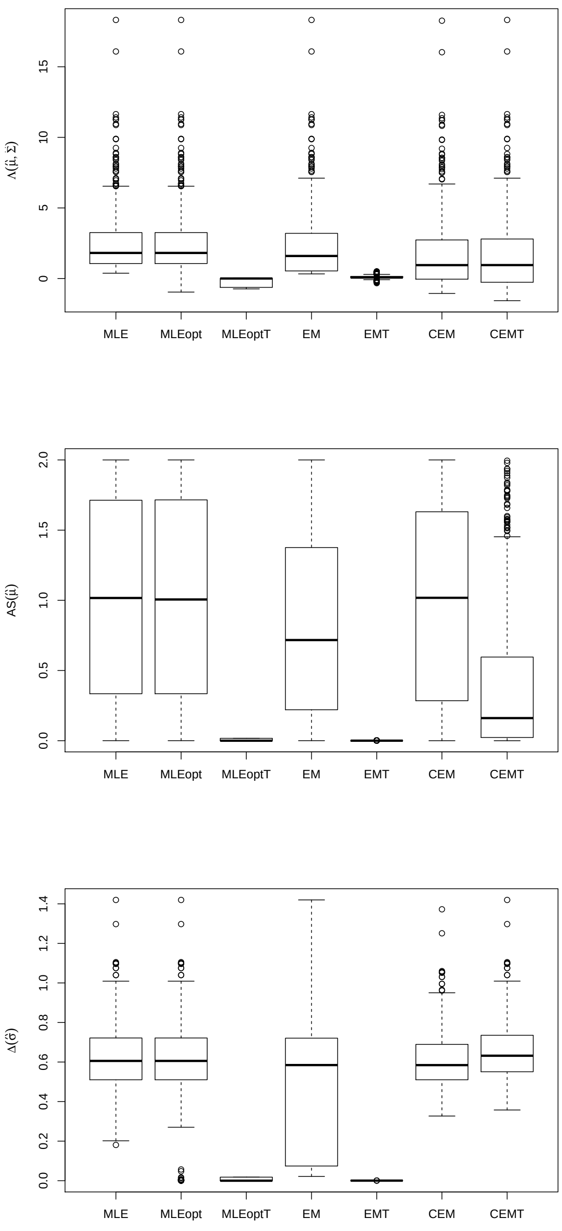


Figure SM–12: Performance of the estimators in the univariate case $p = 1$, sample size $n = 10$, $\sigma = 2\pi$.

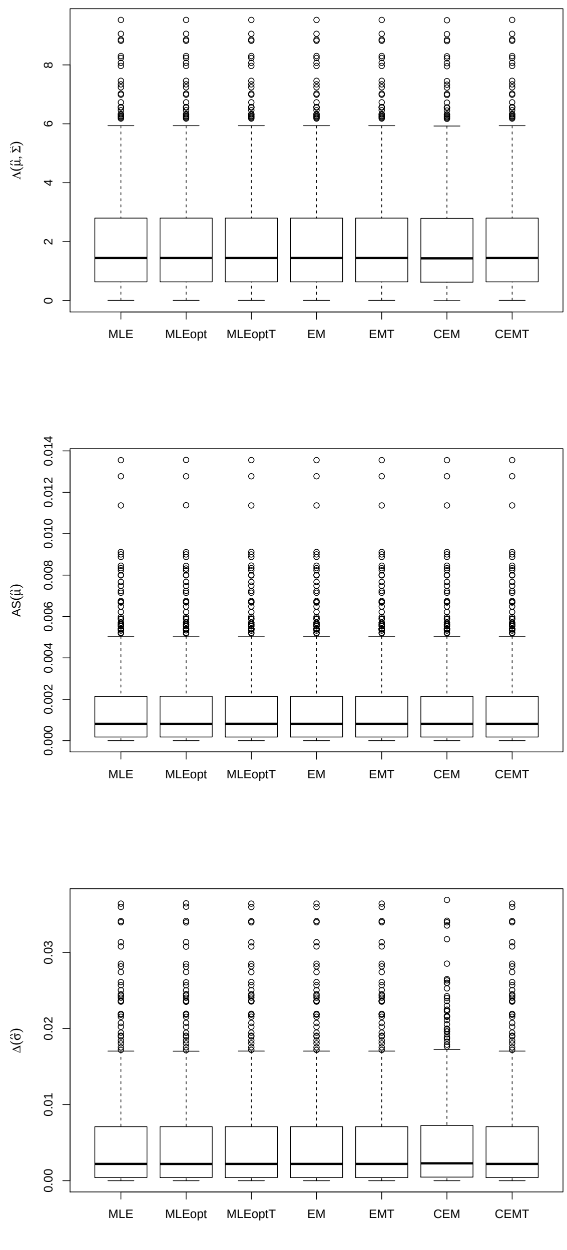


Figure SM–13: Performance of the estimators in the univariate case $p = 1$, sample size $n = 50$, $\sigma = \pi/8$.

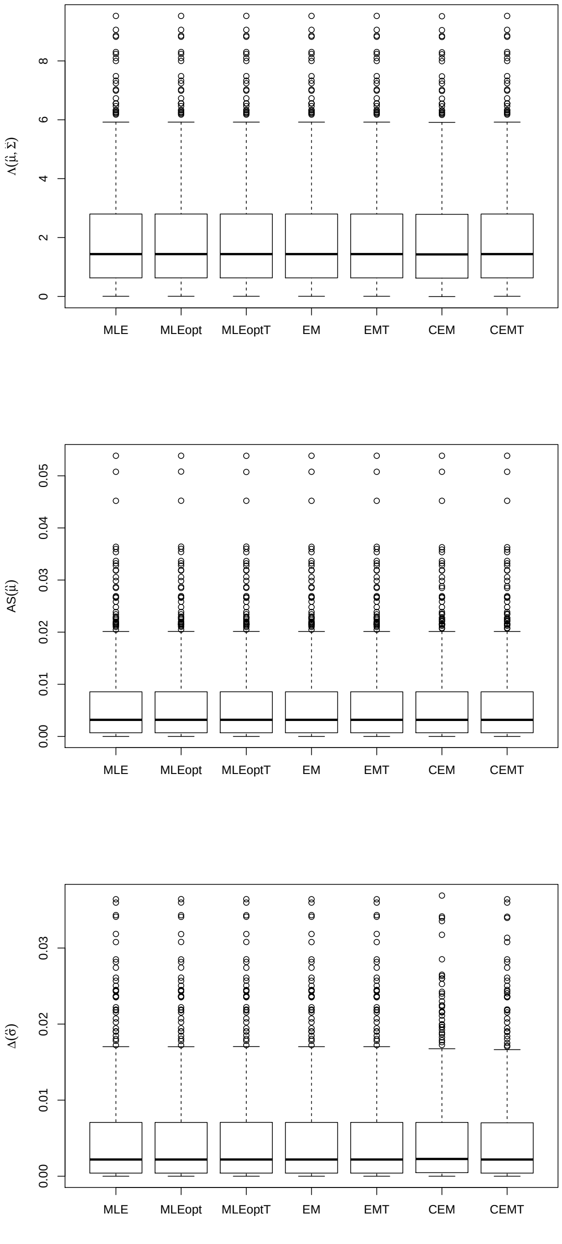


Figure SM–14: Performance of the estimators in the univariate case $p = 1$, sample size $n = 50$, $\sigma = \pi/4$.

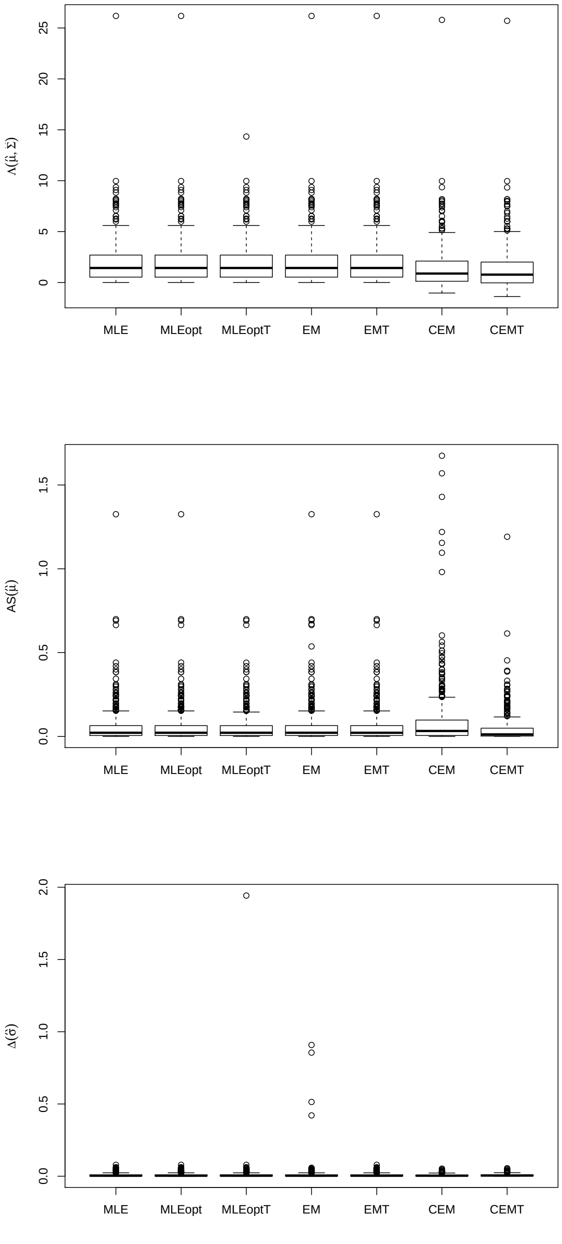


Figure SM–15: Performance of the estimators in the univariate case $p = 1$, sample size $n = 50$, $\sigma = \pi/2$.

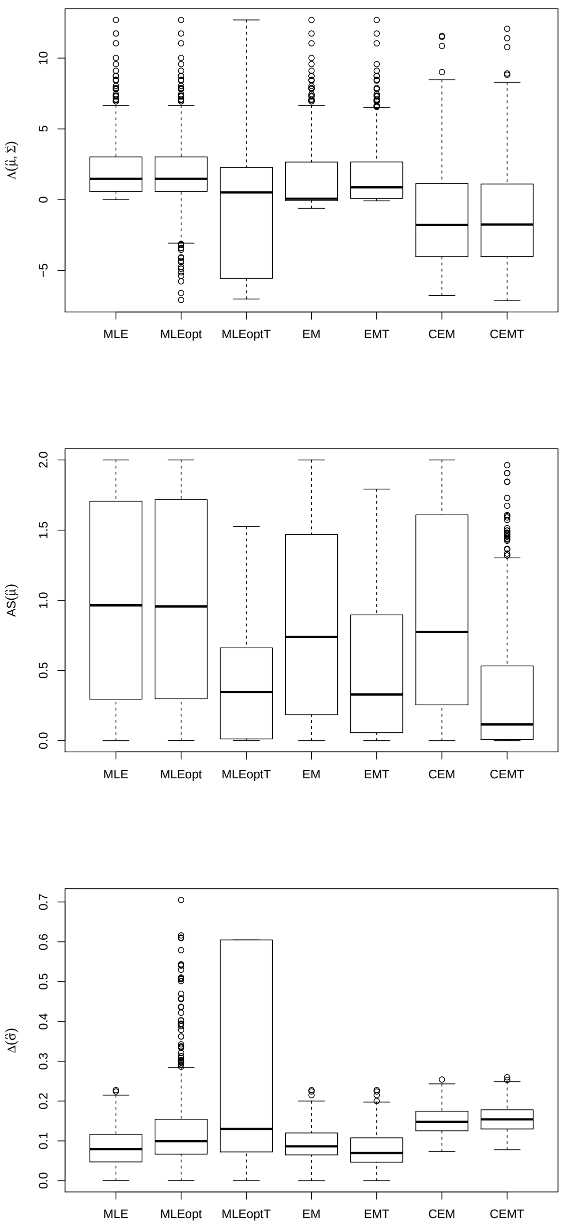


Figure SM–16: Performance of the estimators in the univariate case $p = 1$, sample size $n = 50$, $\sigma = \pi$.

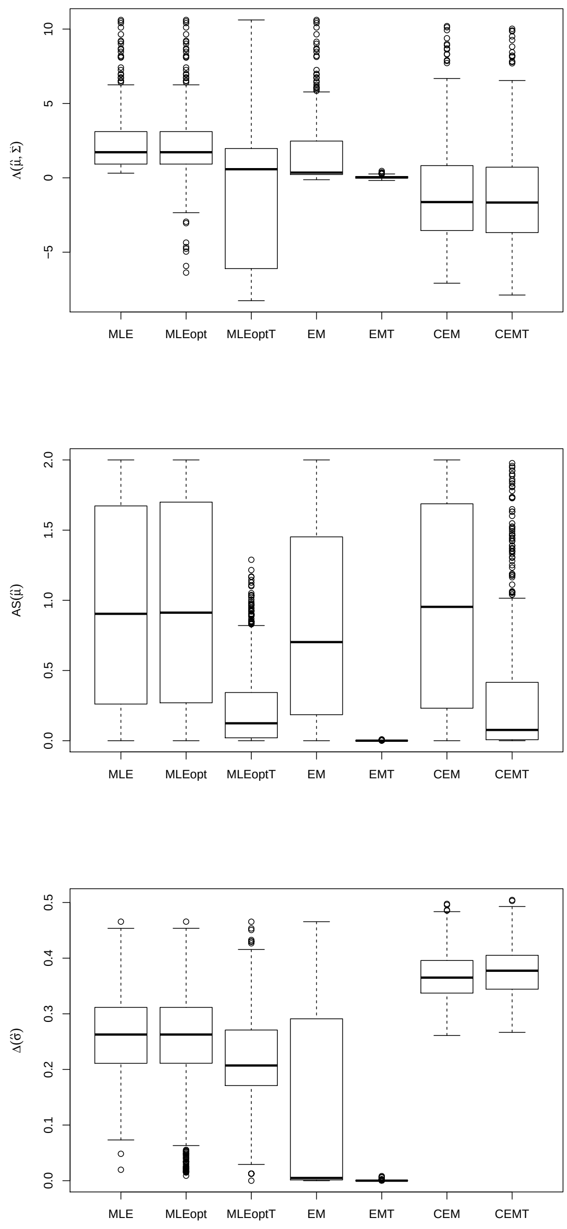


Figure SM–17: Performance of the estimators in the univariate case $p = 1$, sample size $n = 50$, $\sigma = 3\pi/2$.

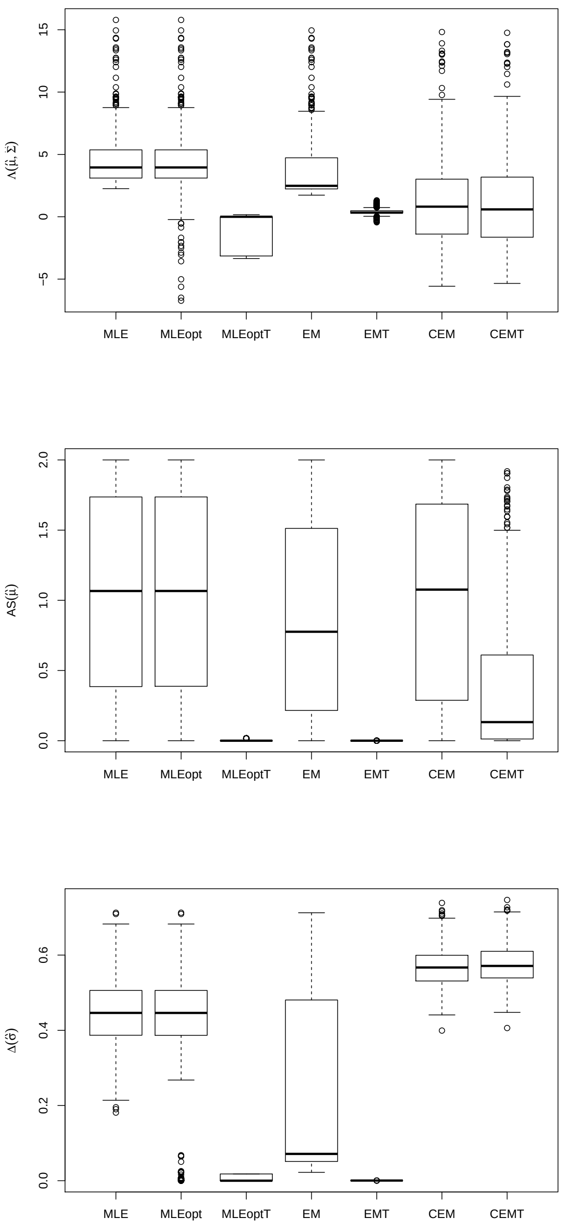


Figure SM–18: Performance of the estimators in the univariate case $p = 1$, sample size $n = 50$, $\sigma = 2\pi$.

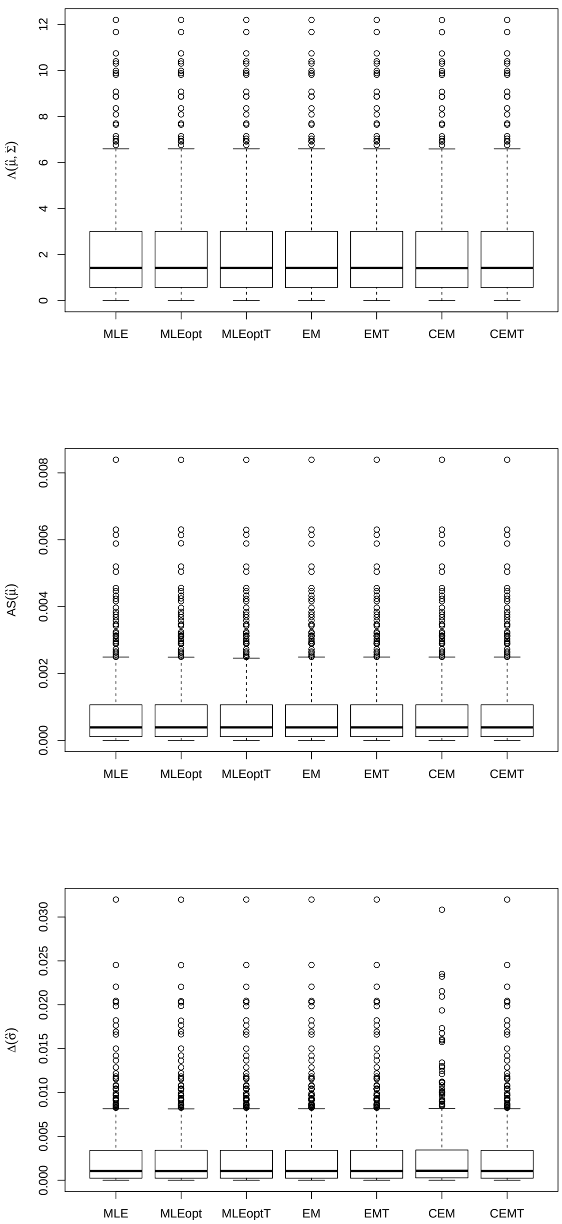


Figure SM–19: Performance of the estimators in the univariate case $p = 1$, sample size $n = 100$, $\sigma = \pi/8$.

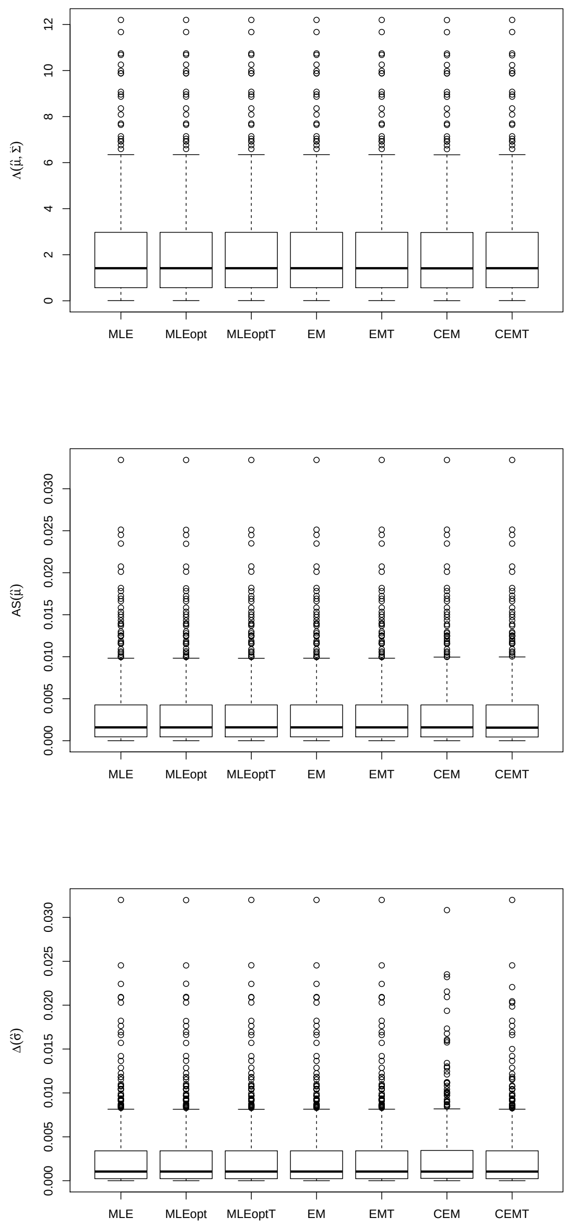


Figure SM–20: Performance of the estimators in the univariate case $p = 1$, sample size $n = 100$, $\sigma = \pi/4$.

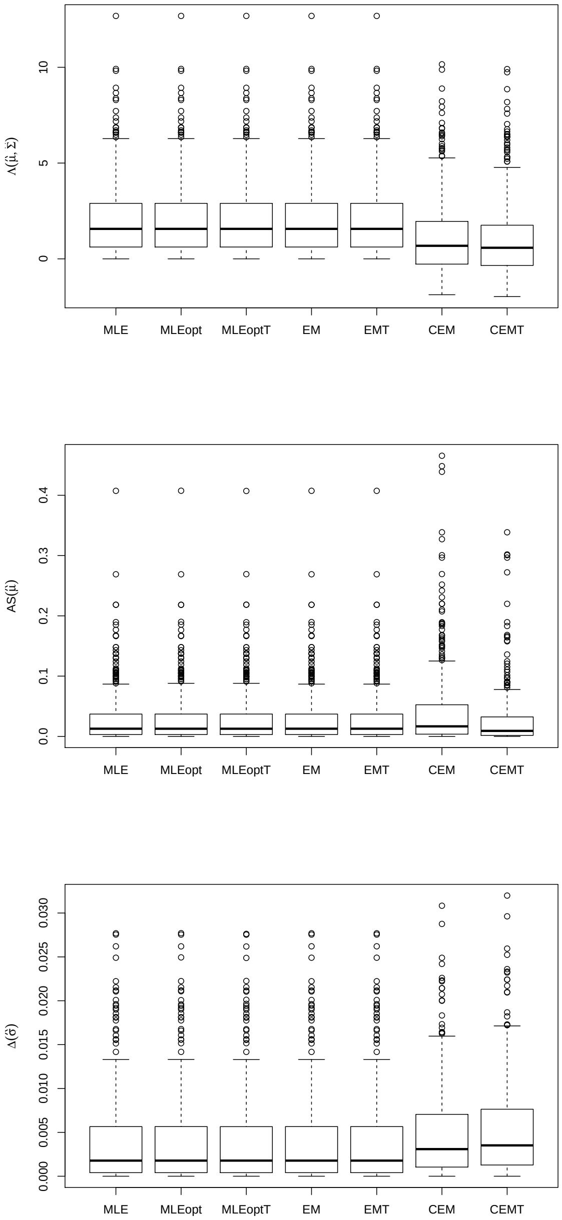


Figure SM–21: Performance of the estimators in the univariate case $p = 1$, sample size $n = 100$, $\sigma = \pi/2$.

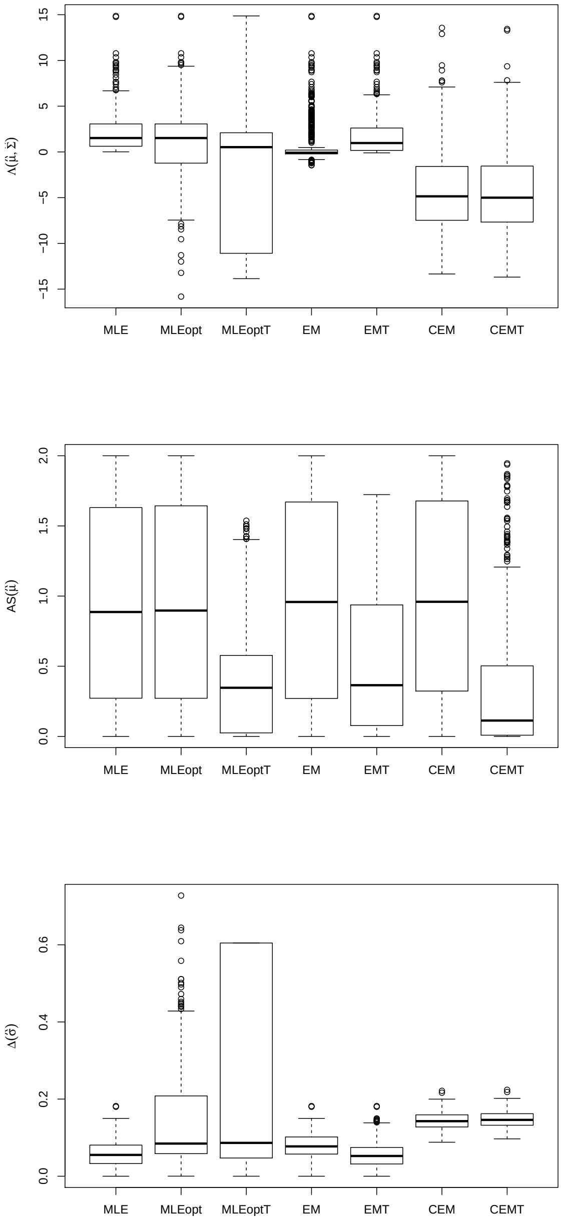


Figure SM–22: Performance of the estimators in the univariate case $p = 1$, sample size $n = 100$, $\sigma = \pi$.

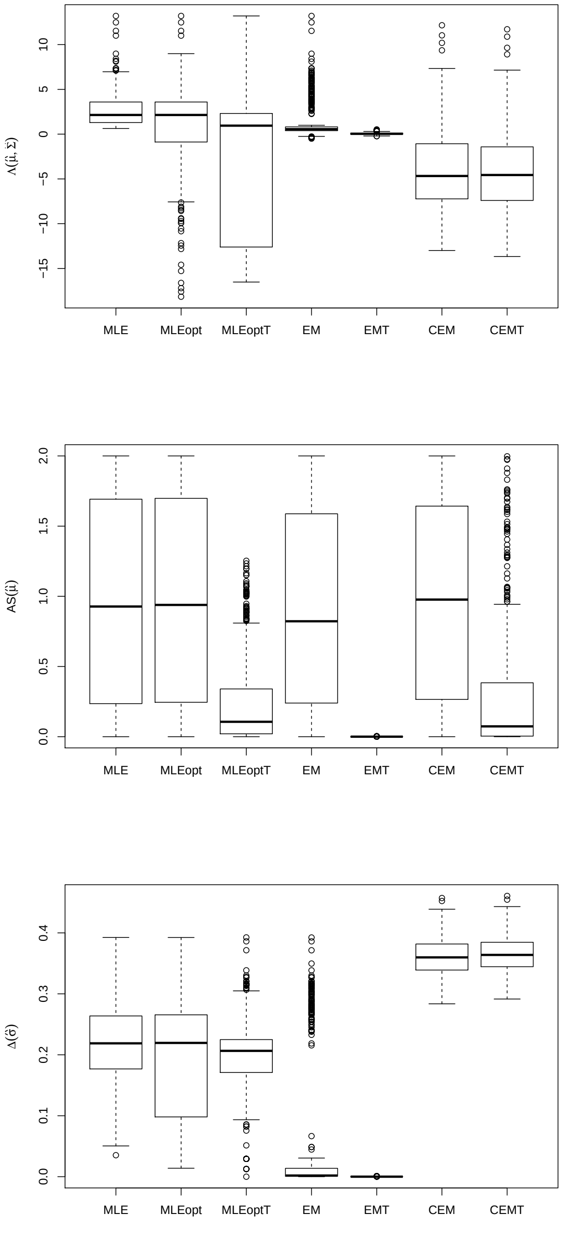


Figure SM–23: Performance of the estimators in the univariate case $p = 1$, sample size $n = 100$, $\sigma = 3\pi/2$.

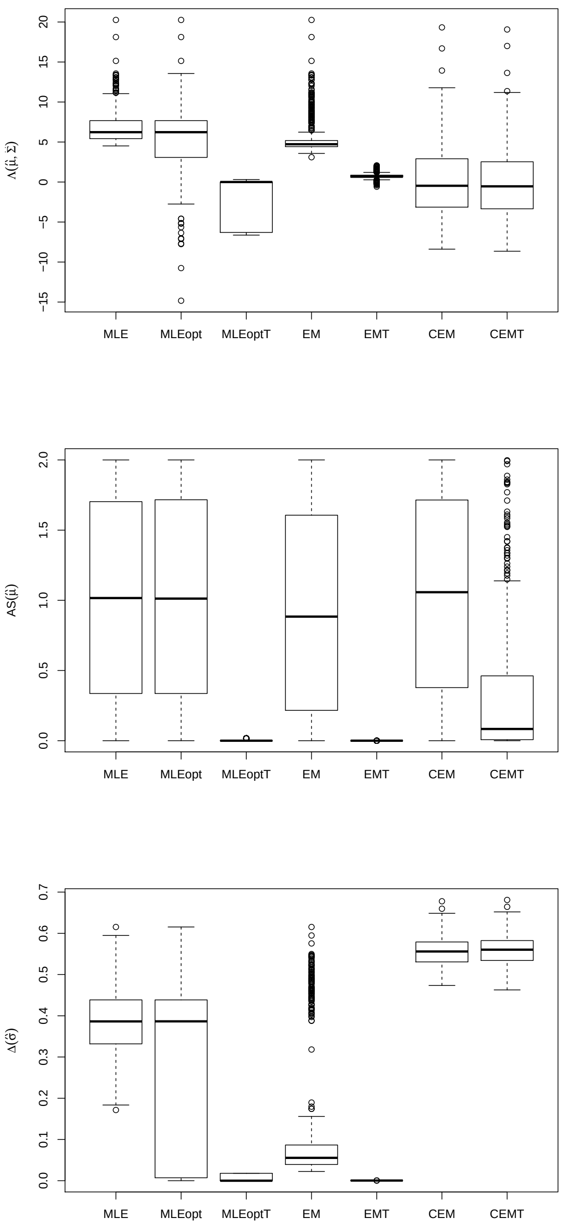


Figure SM–24: Performance of the estimators in the univariate case $p = 1$, sample size $n = 100$, $\sigma = 2\pi$.

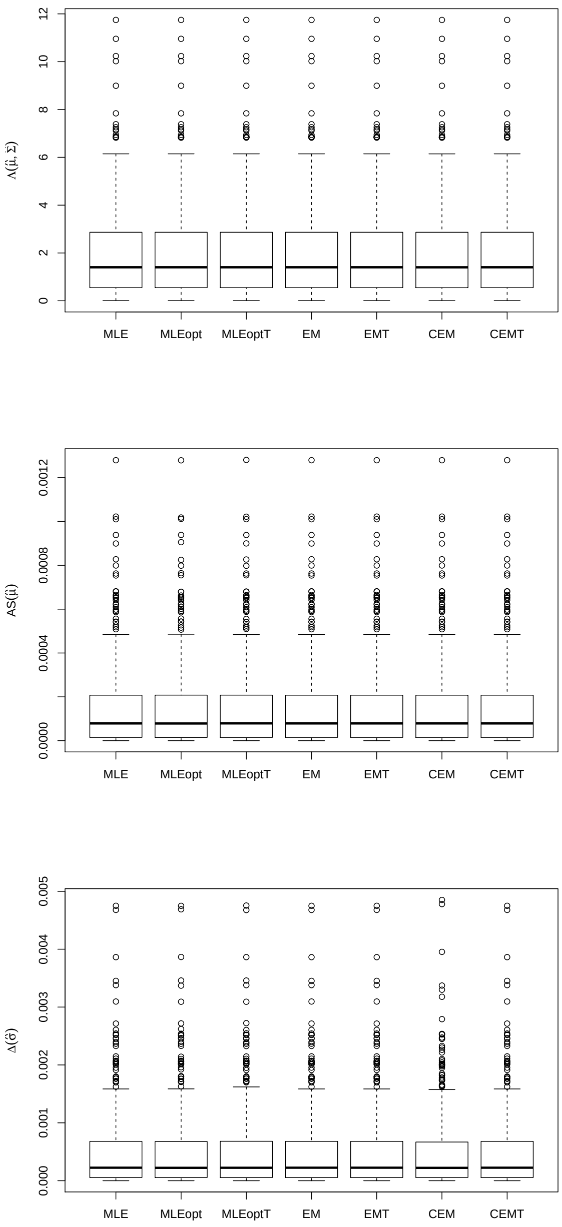


Figure SM–25: Performance of the estimators in the univariate case $p = 1$, sample size $n = 500$, $\sigma = \pi/8$.

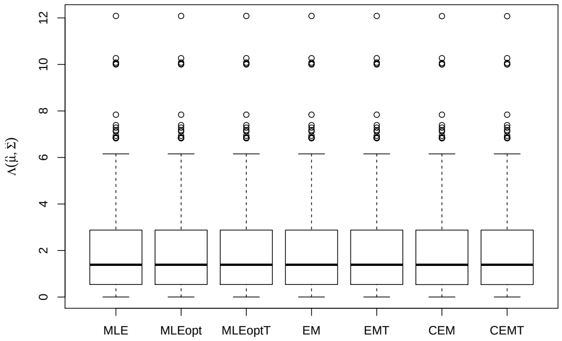


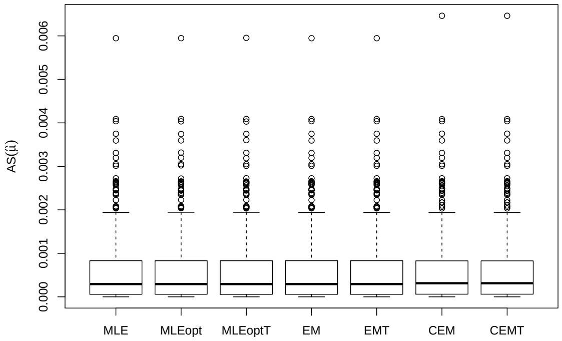


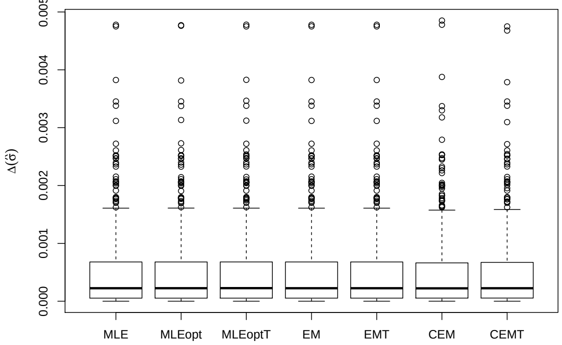


Figure SM–26: Performance of the estimators in the univariate case $p = 1$, sample size $n = 500$, $\sigma = \pi/4$.

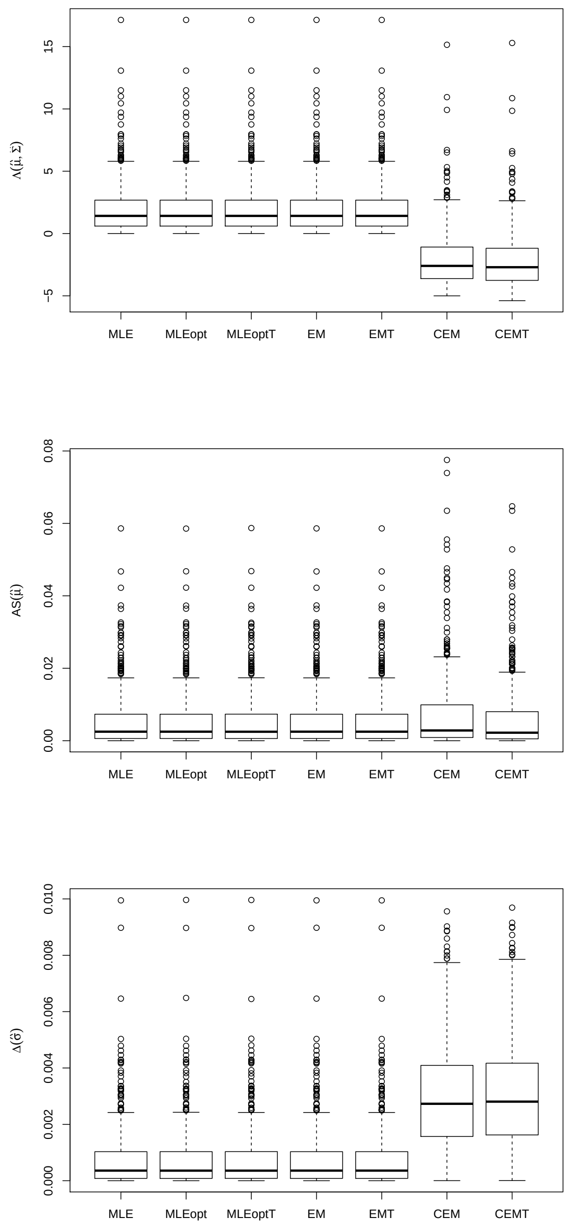


Figure SM–27: Performance of the estimators in the univariate case $p = 1$, sample size $n = 500$, $\sigma = \pi/2$.

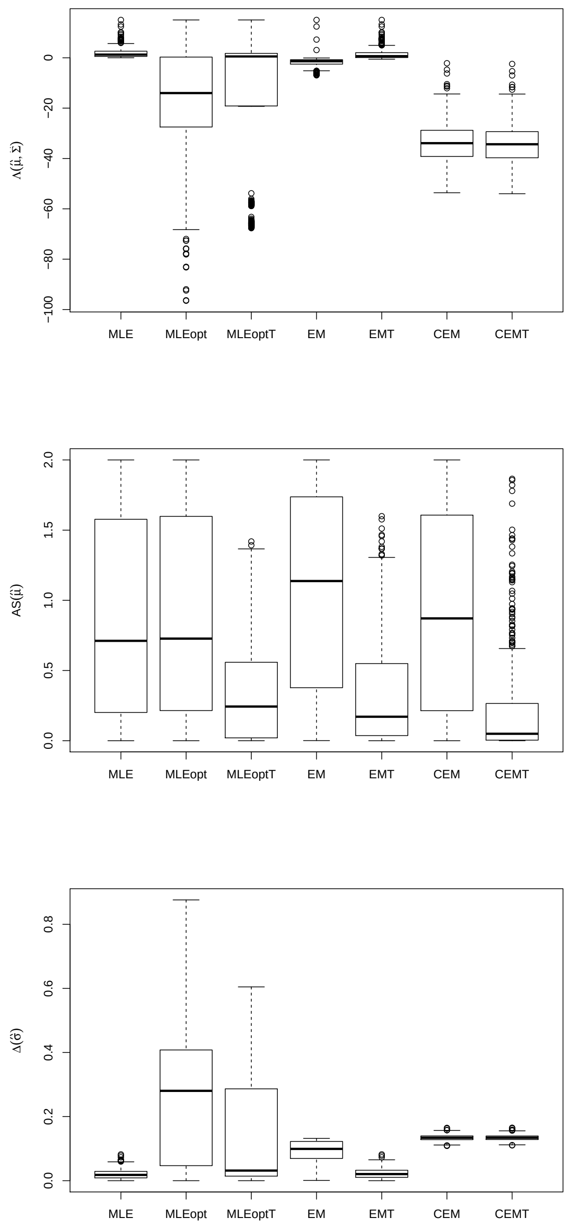


Figure SM–28: Performance of the estimators in the univariate case $p = 1$, sample size $n = 500$, $\sigma = \pi$.

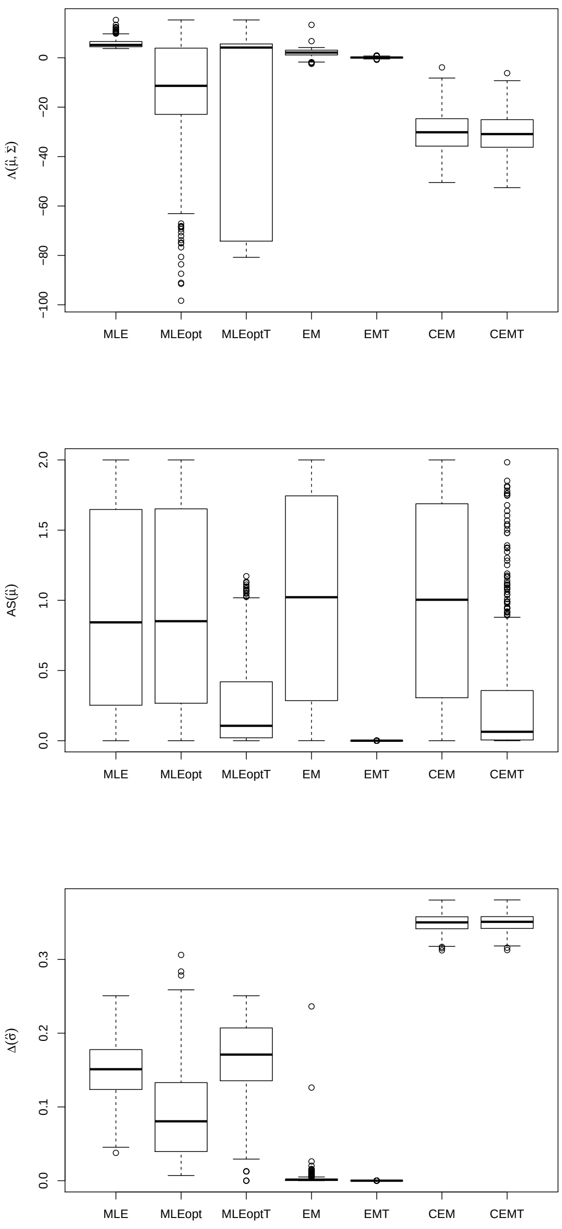


Figure SM–29: Performance of the estimators in the univariate case $p = 1$, sample size $n = 500$, $\sigma = 3\pi/2$.

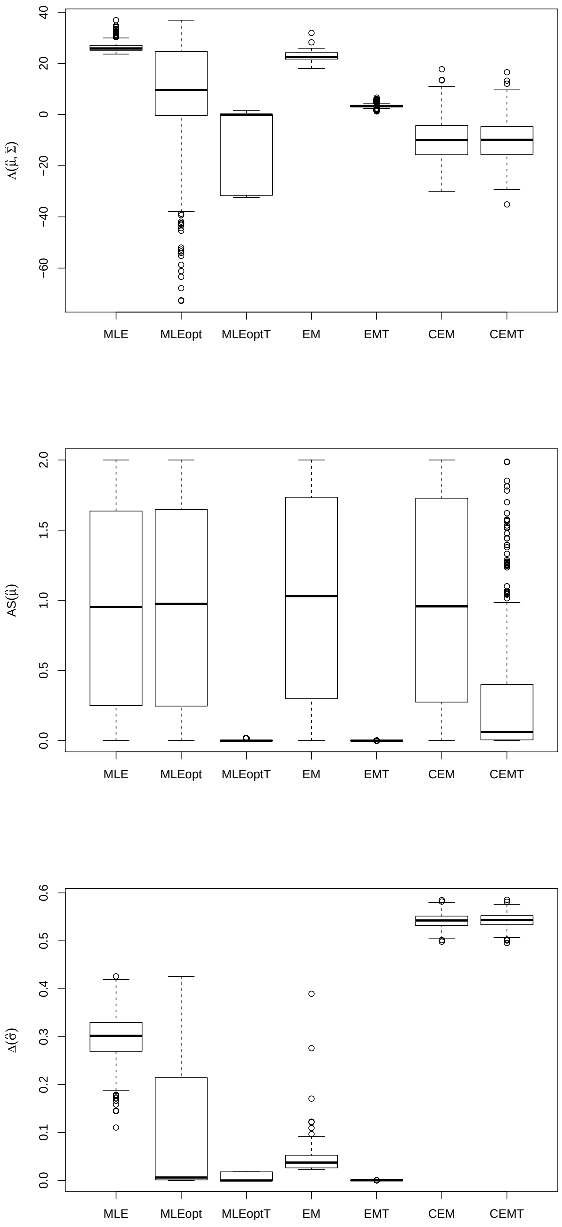


Figure SM–30: Performance of the estimators in the univariate case $p = 1$, sample size $n = 500$, $\sigma = 2\pi$.

### SM–4.2 $p = 2$

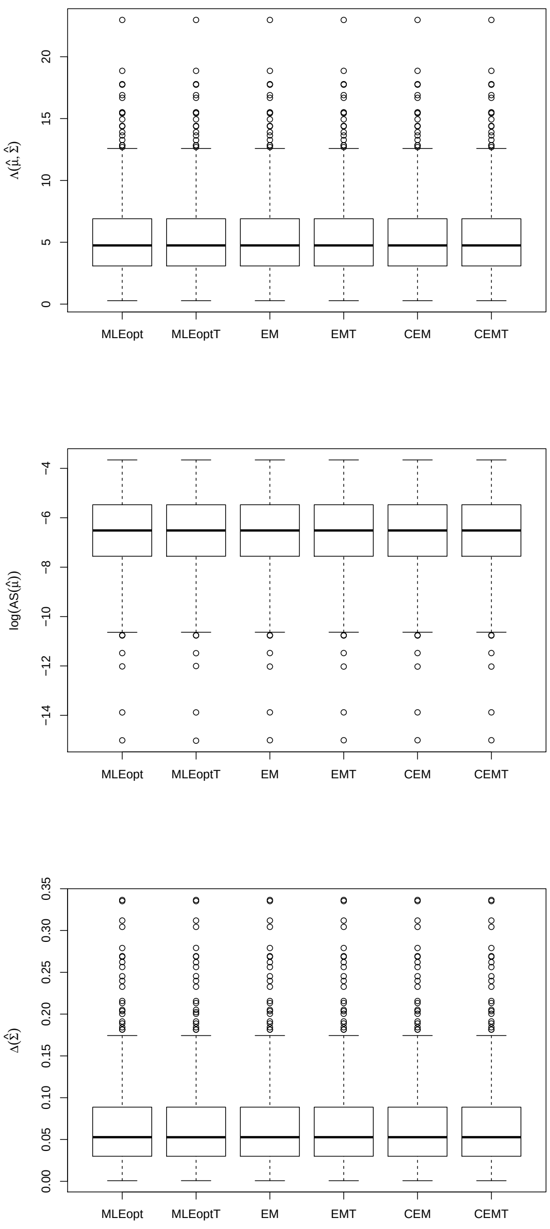


Figure SM–31: Performance of the estimators in the bivariate case $p = 2$, sample size $n = 50$, $\sigma = \pi/8$.

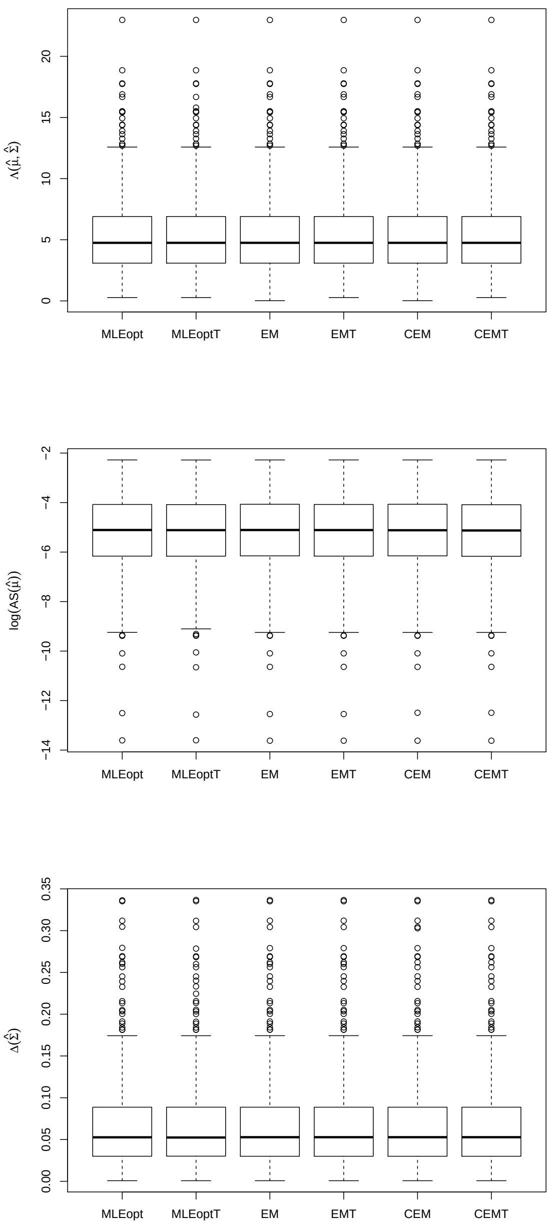


Figure SM–32: Performance of the estimators in the bivariate case $p = 2$, sample size $n = 50$, $\sigma = \pi/4$.

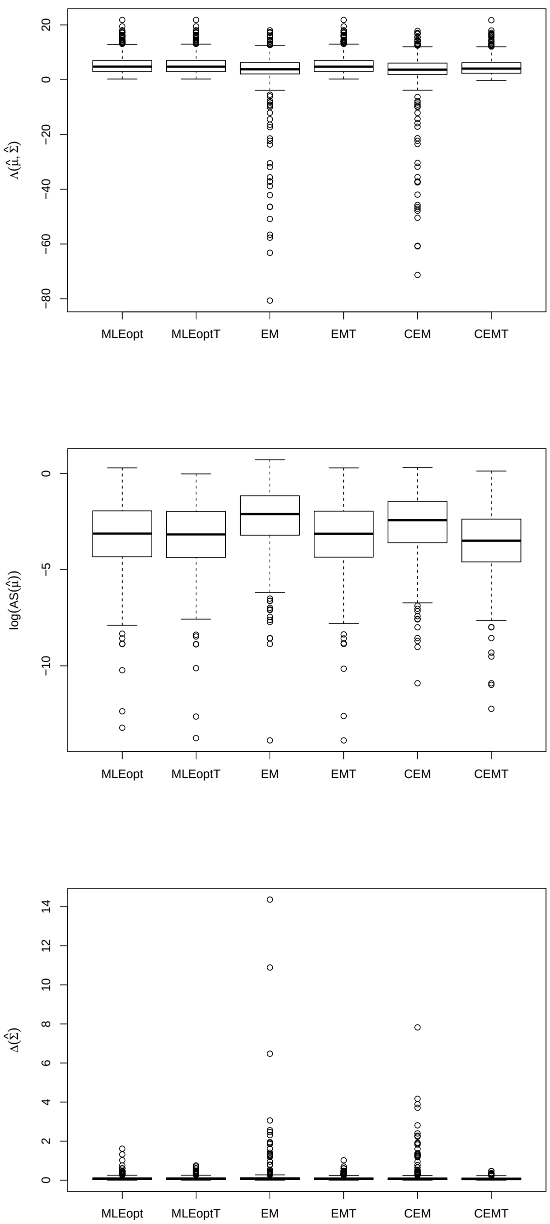


Figure SM–33: Performance of the estimators in the bivariate case $p = 2$, sample size $n = 50$, $\sigma = \pi/2$.

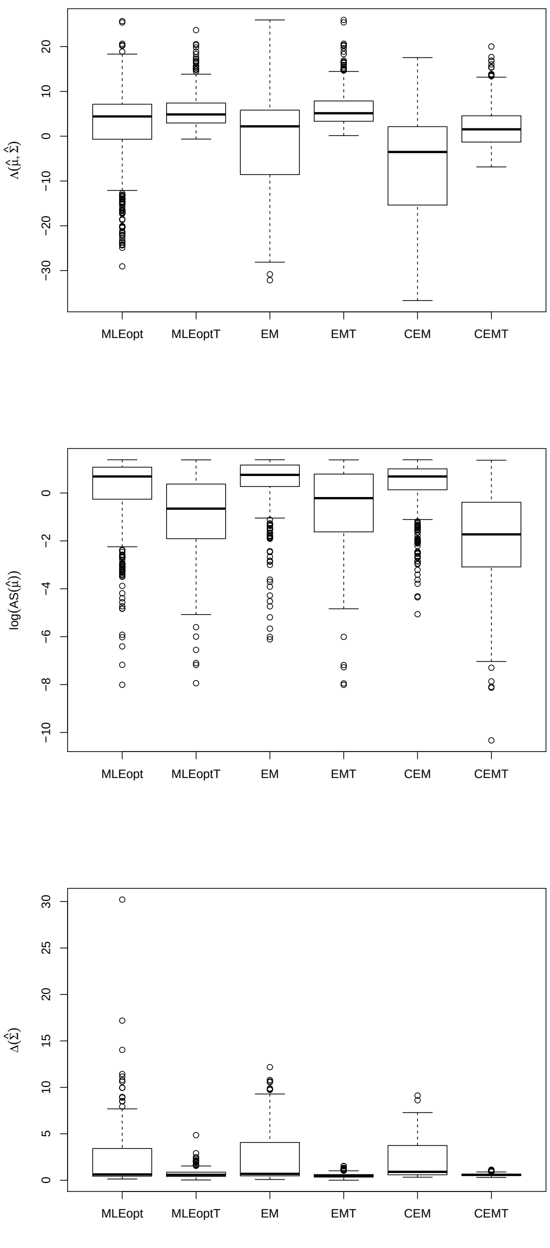


Figure SM–34: Performance of the estimators in the bivariate case $p = 2$, sample size $n = 50$, $\sigma = \pi$.

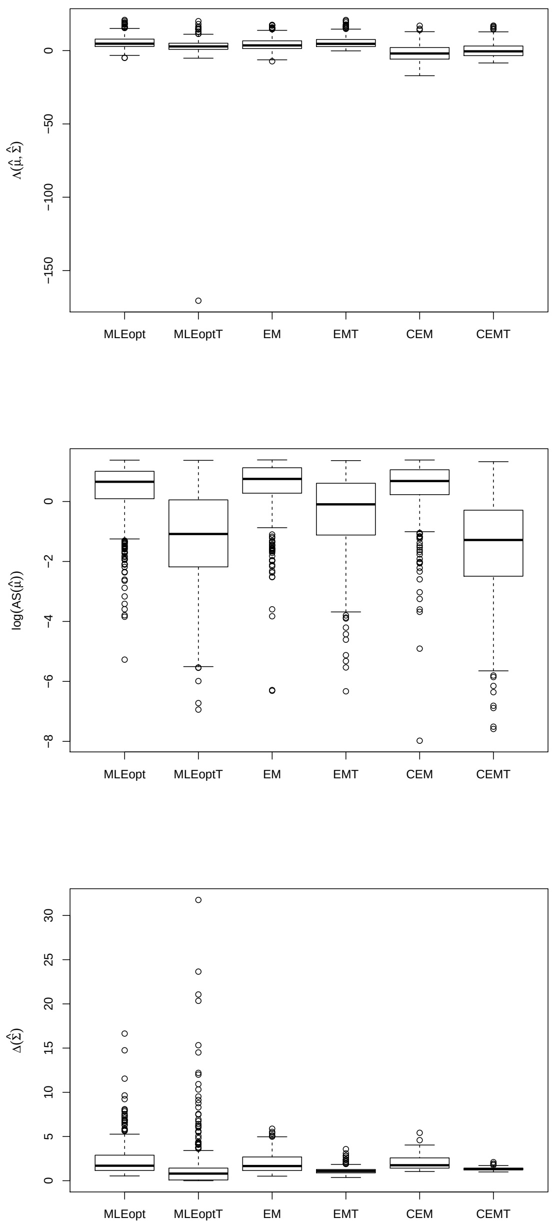


Figure SM–35: Performance of the estimators in the bivariate case $p = 2$, sample size $n = 50$, $\sigma = 3\pi/2$.

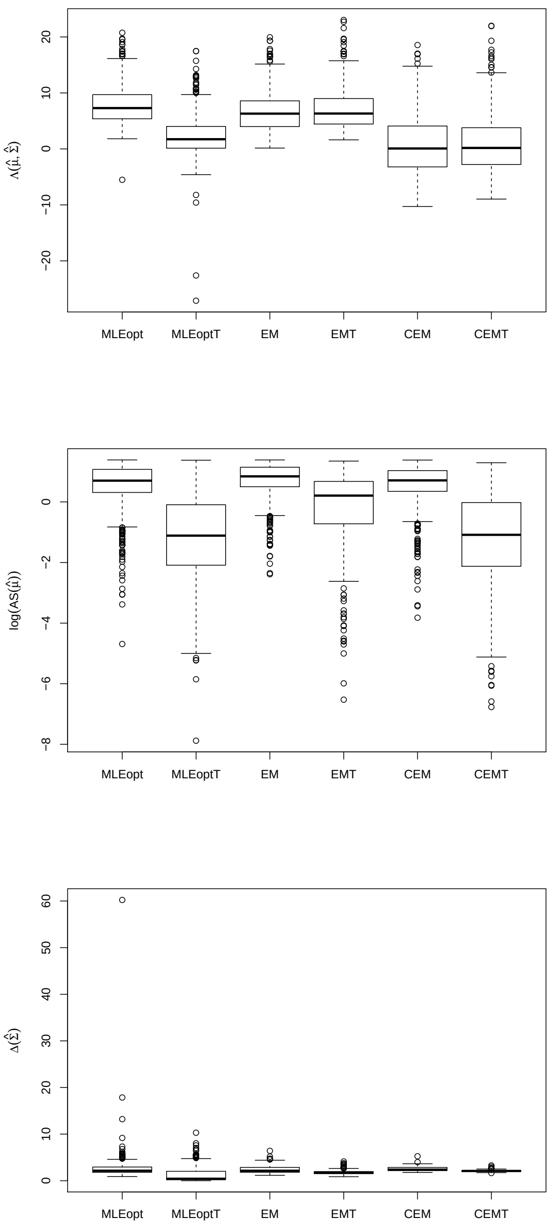


Figure SM–36: Performance of the estimators in the bivariate case $p = 2$, sample size $n = 50$, $\sigma = 2\pi$.

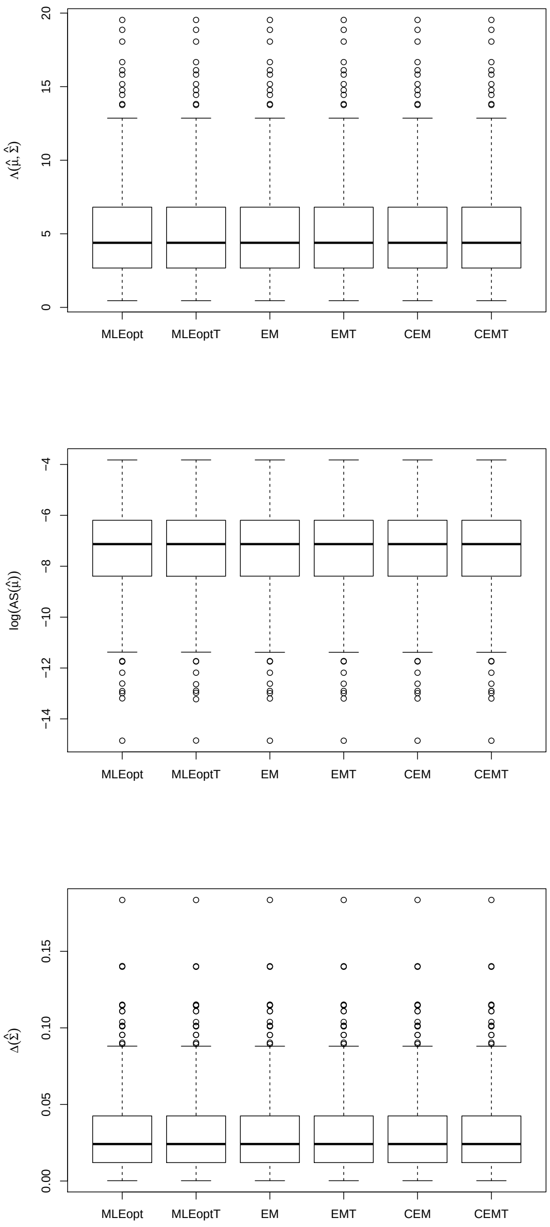


Figure SM–37: Performance of the estimators in the bivariate case $p = 2$, sample size $n = 100$, $\sigma = \pi/8$.

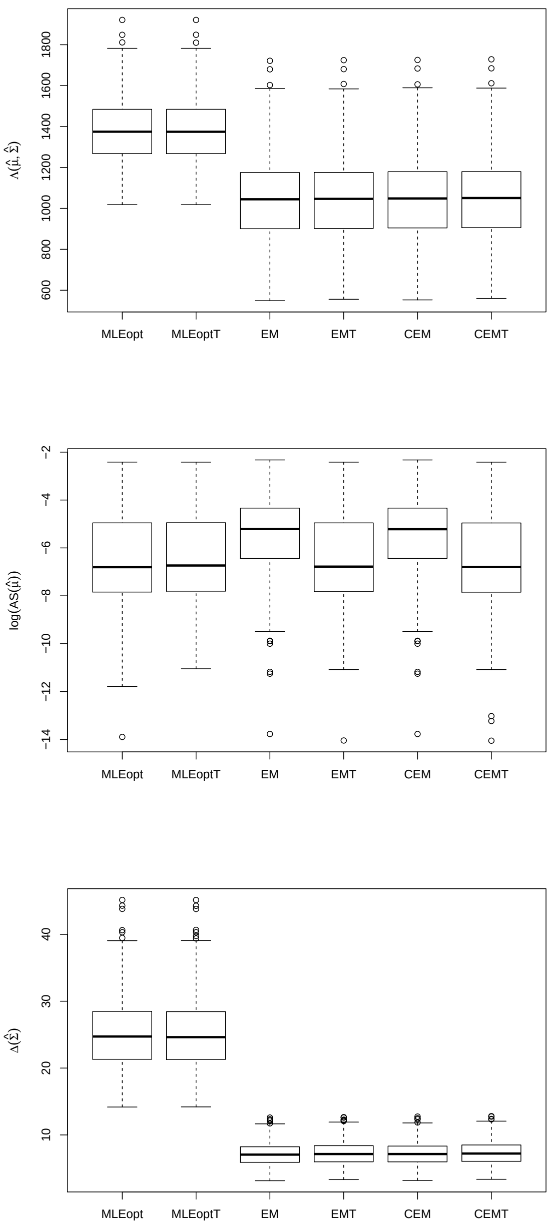


Figure SM–38: Performance of the estimators in the bivariate case $p = 2$, sample size $n = 100$, $\sigma = \pi/4$.

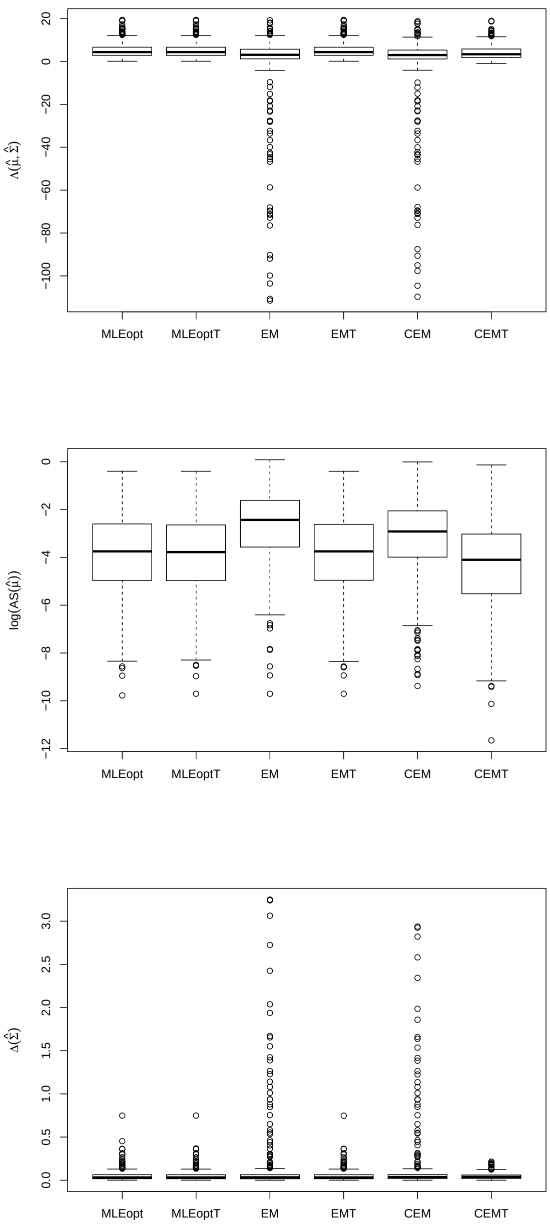


Figure SM–39: Performance of the estimators in the bivariate case $p = 2$, sample size $n = 100$, $\sigma = \pi/2$.

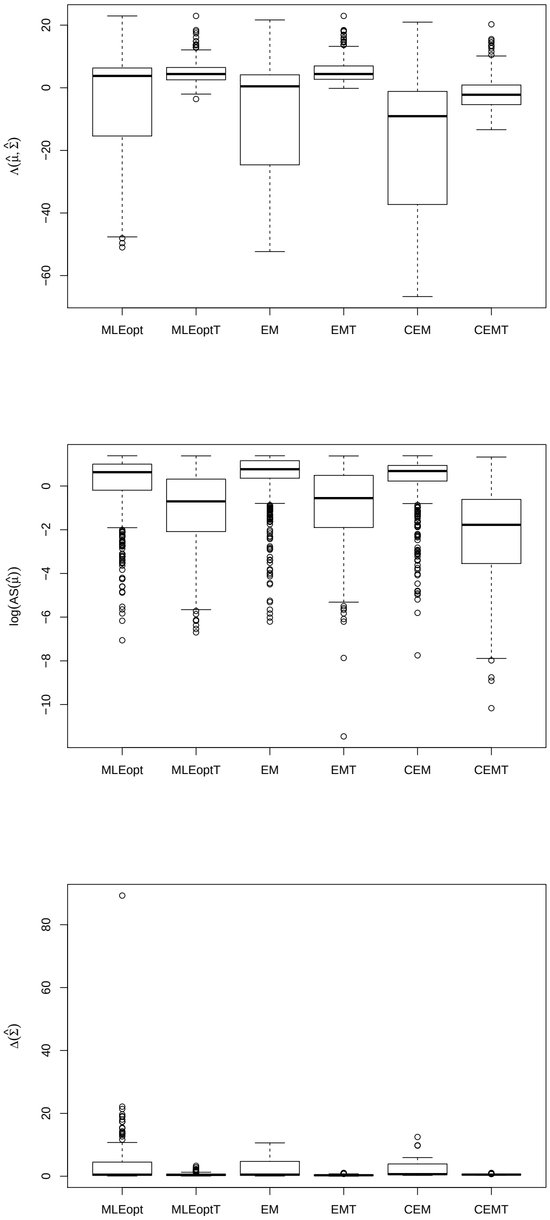


Figure SM–40: Performance of the estimators in the bivariate case $p = 2$, sample size $n = 100$, $\sigma = \pi$.

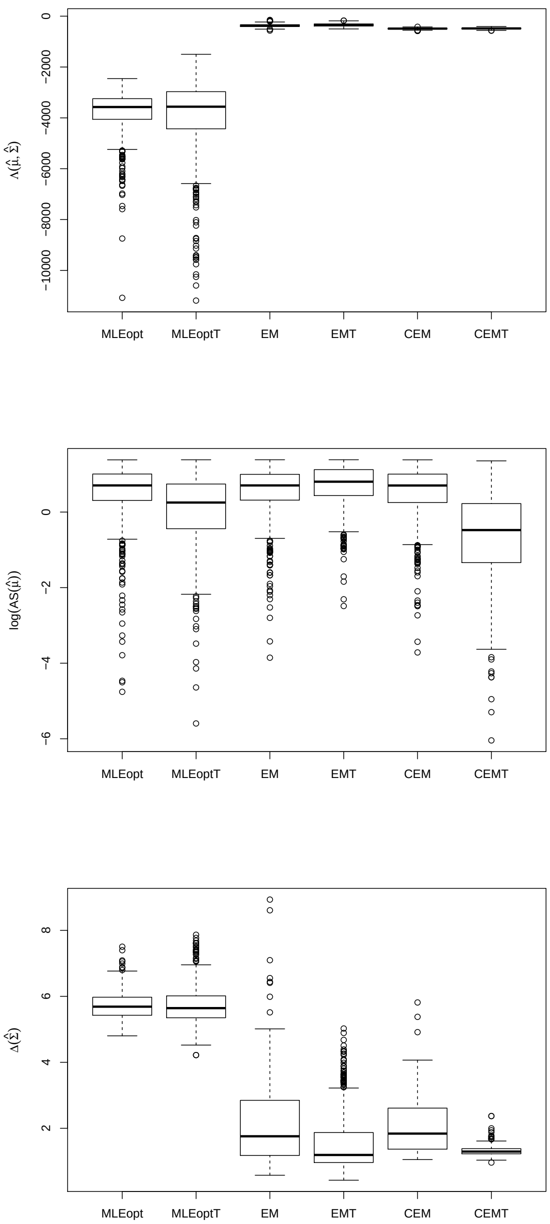


Figure SM–41: Performance of the estimators in the bivariate case $p = 2$, sample size $n = 100$, $\sigma = 3\pi/2$.

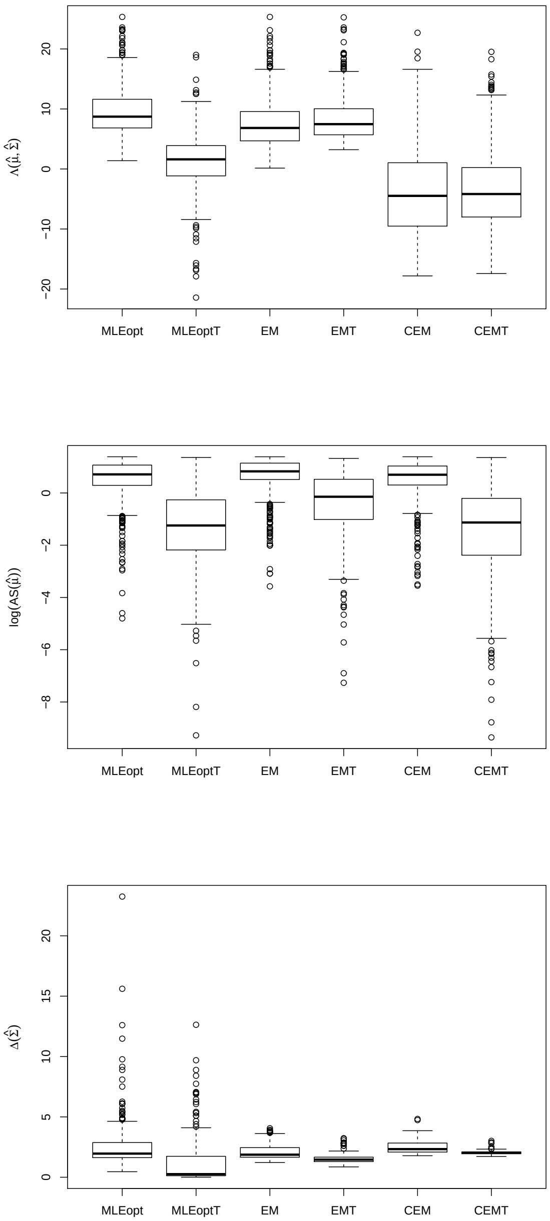


Figure SM–42: Performance of the estimators in the bivariate case $p = 2$, sample size $n = 100$, $\sigma = 2\pi$.

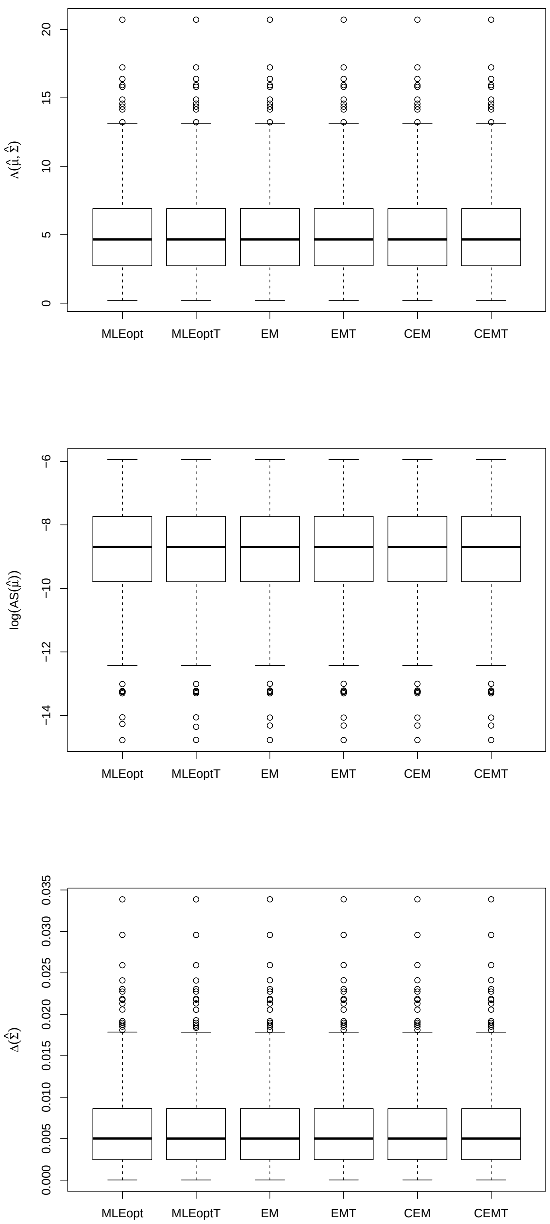


Figure SM–43: Performance of the estimators in the bivariate case $p = 2$, sample size $n = 500$, $\sigma = \pi/8$.

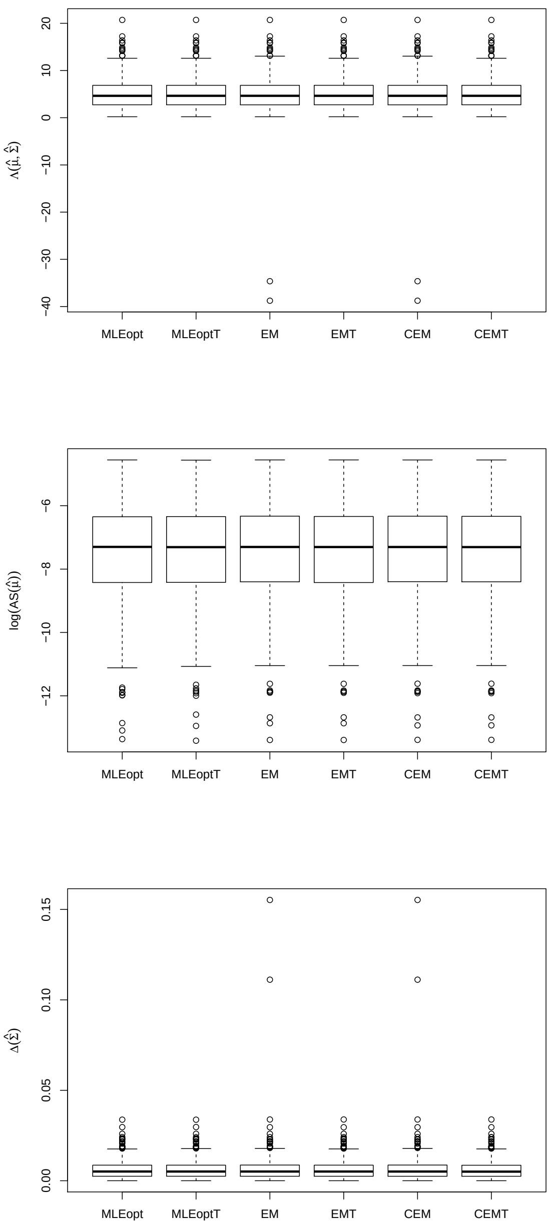


Figure SM–44: Performance of the estimators in the bivariate case $p = 2$, sample size $n = 500$, $\sigma = \pi/4$.

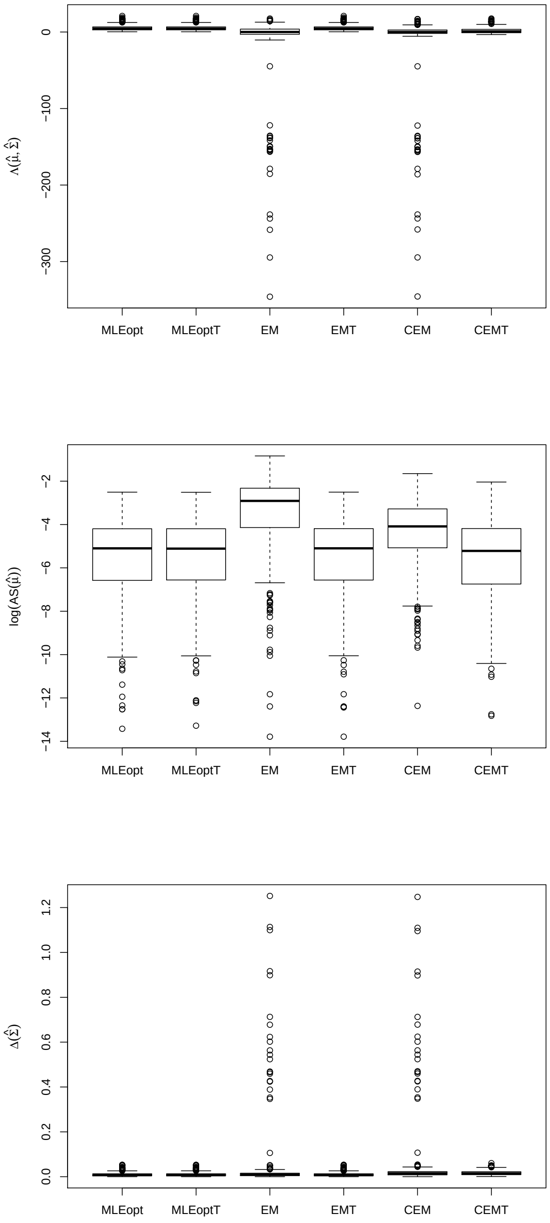


Figure SM–45: Performance of the estimators in the bivariate case $p = 2$, sample size $n = 500$, $\sigma = \pi/2$.

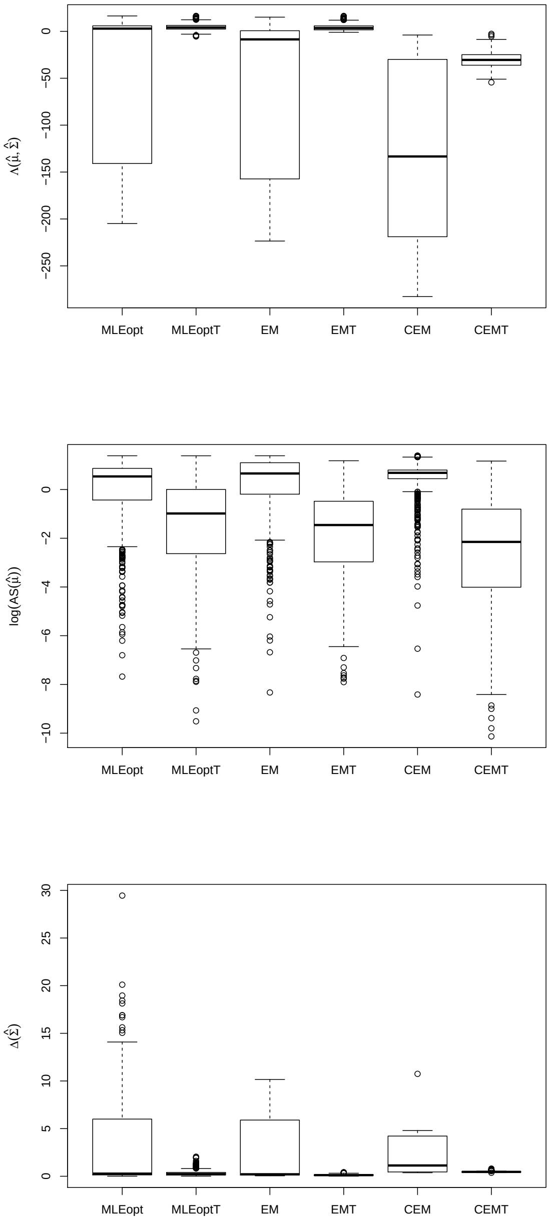


Figure SM–46: Performance of the estimators in the bivariate case $p = 2$, sample size $n = 500$, $\sigma = \pi$.

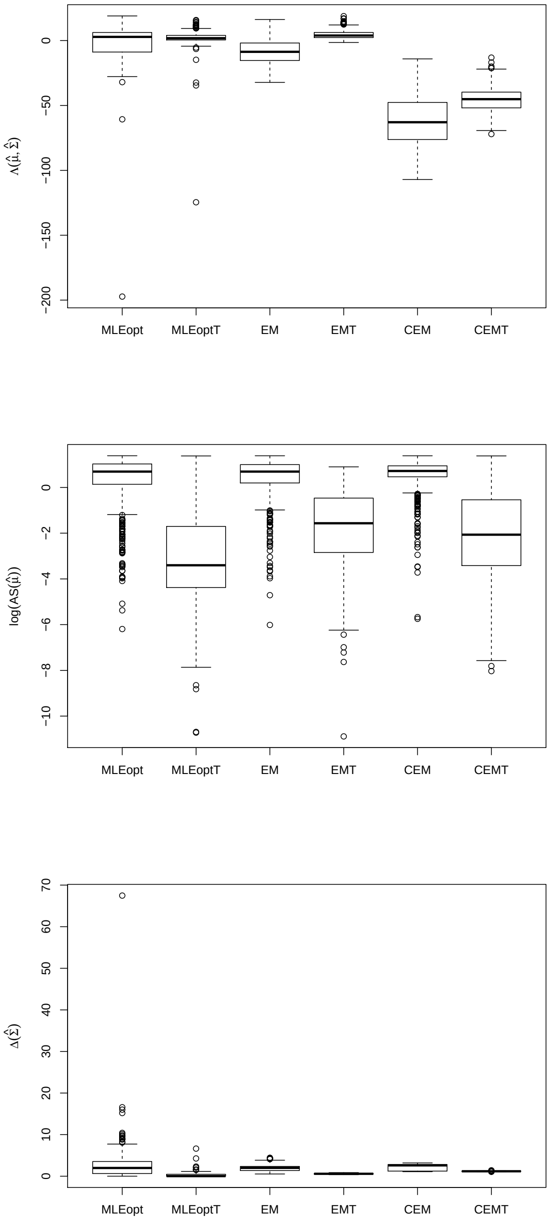


Figure SM–47: Performance of the estimators in the bivariate case $p = 2$, sample size $n = 500$, $\sigma = 3\pi/2$.

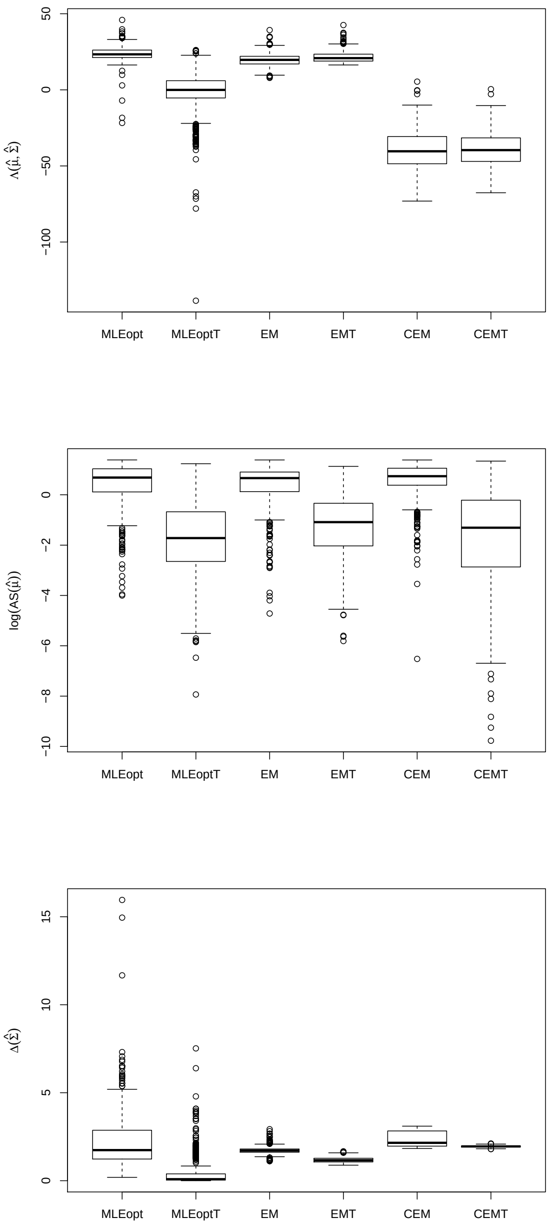


Figure SM–48: Performance of the estimators in the bivariate case $p = 2$, sample size $n = 500$, $\sigma = 2\pi$.

### SM–4.3 $p = 5$

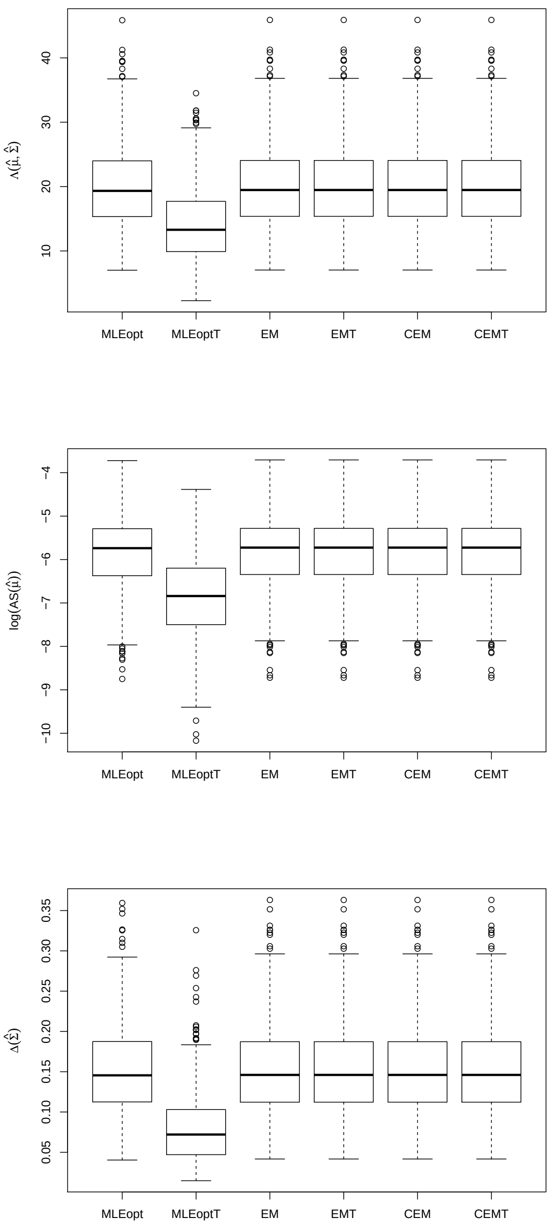


Figure SM–49: Performance of the estimators in the case $p = 5$, sample size $n = 100$, $\sigma = \pi/8$.

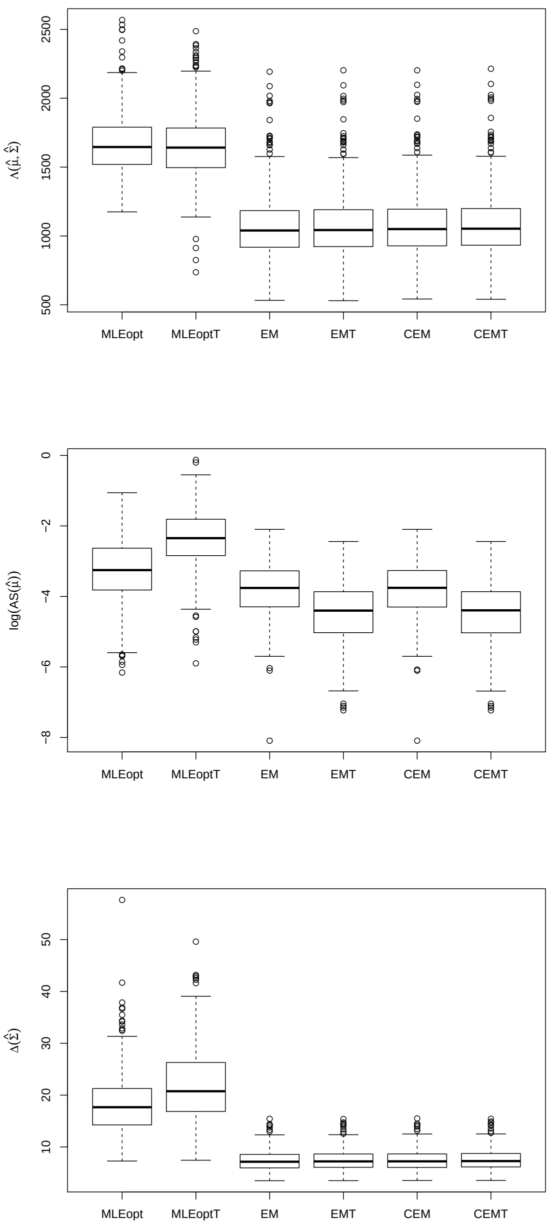


Figure SM–50: Performance of the estimators in the case $p = 5$, sample size $n = 100$, $\sigma = \pi/4$.

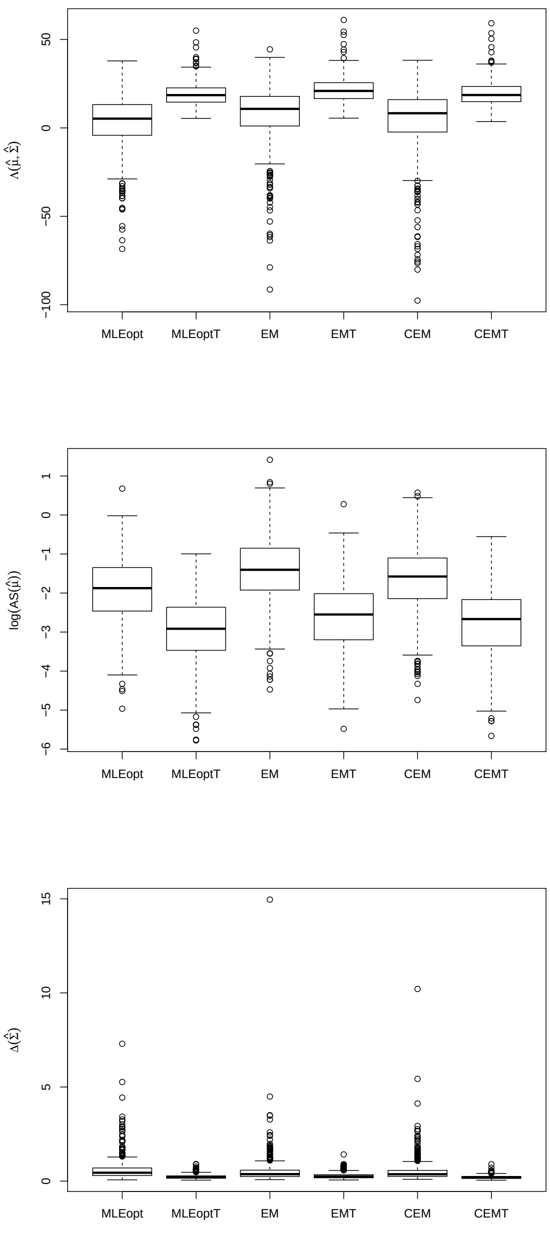


Figure SM–51: Performance of the estimators in the case $p = 5$, sample size $n = 100$, $\sigma = \pi/2$.

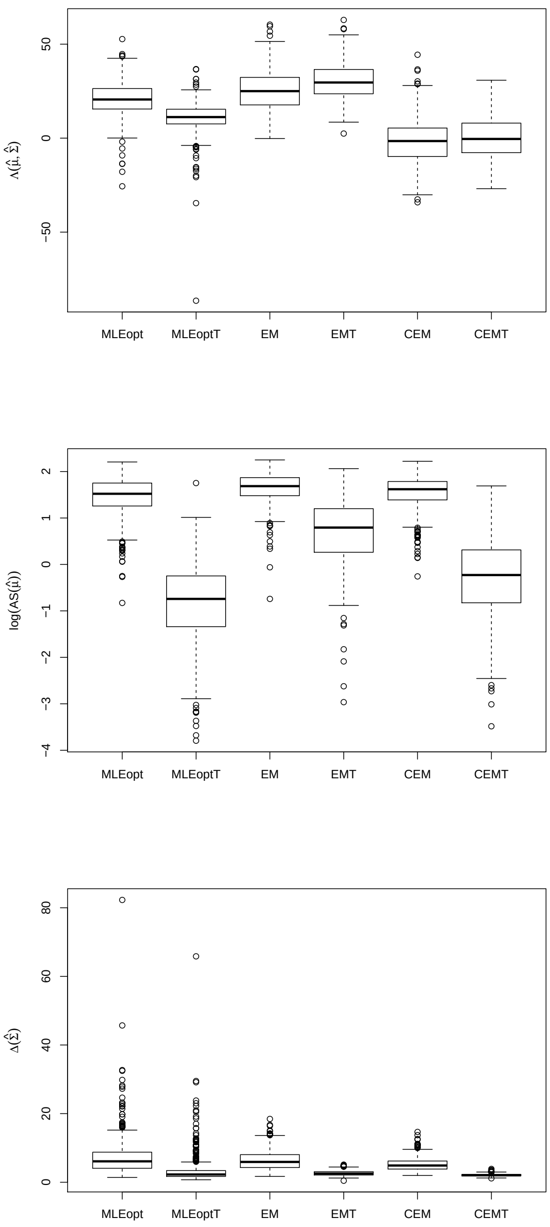


Figure SM–52: Performance of the estimators in the case $p = 5$, sample size $n = 100$, $\sigma = \pi$.

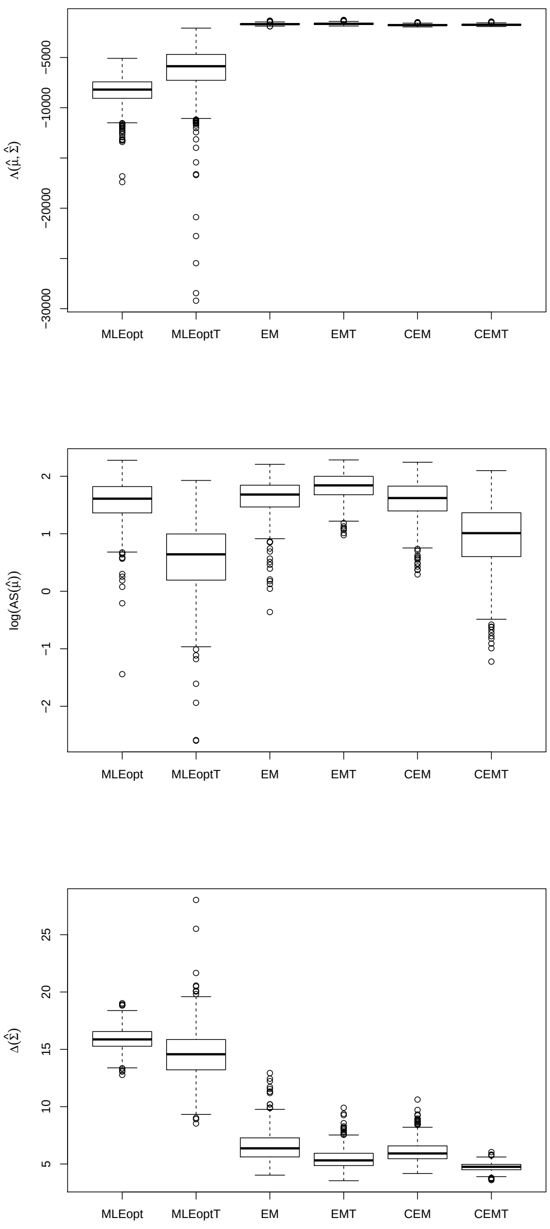


Figure SM–53: Performance of the estimators in the case $p = 5$, sample size $n = 100$, $\sigma = 3\pi/2$.

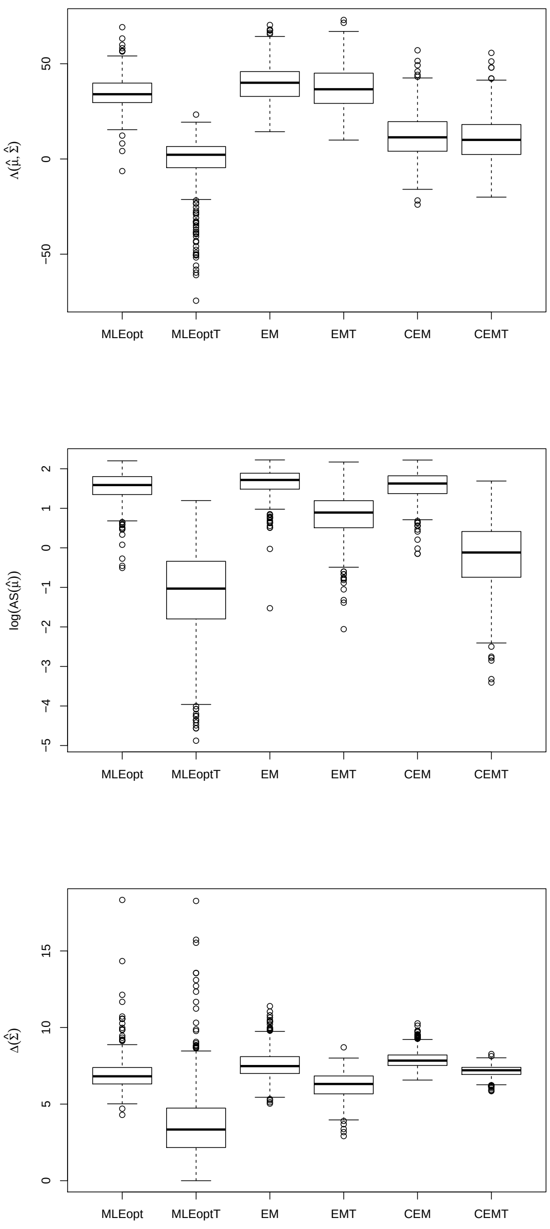


Figure SM–54: Performance of the estimators in the case $p = 5$, sample size $n = 100$, $\sigma = 2\pi$.

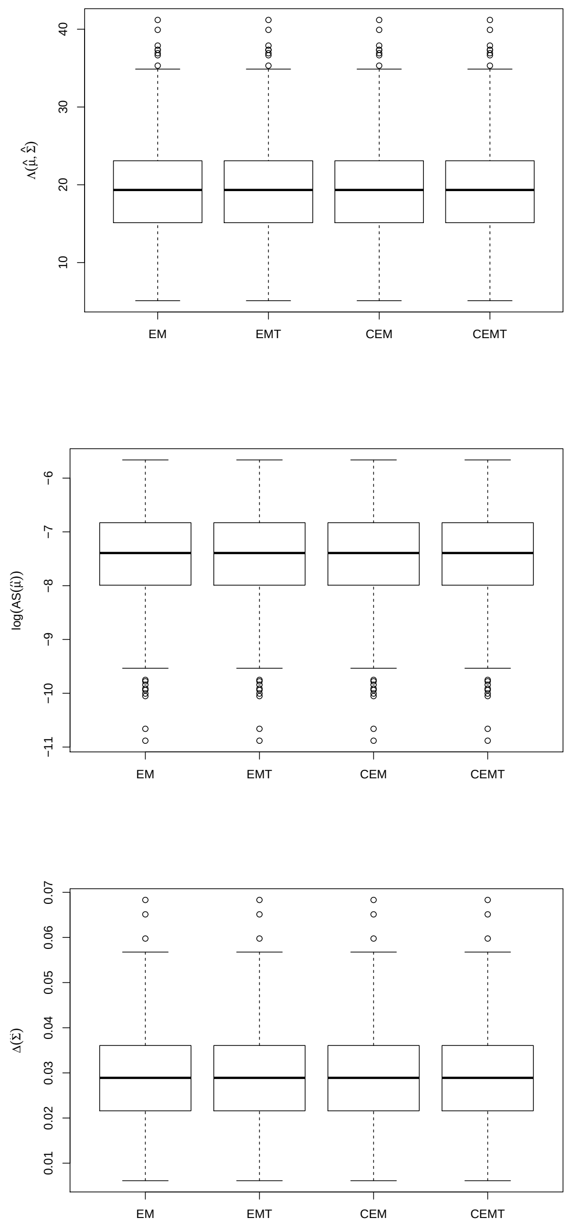


Figure SM–55: Performance of the estimators in the case $p = 5$, sample size $n = 500$, $\sigma = \pi/8$.

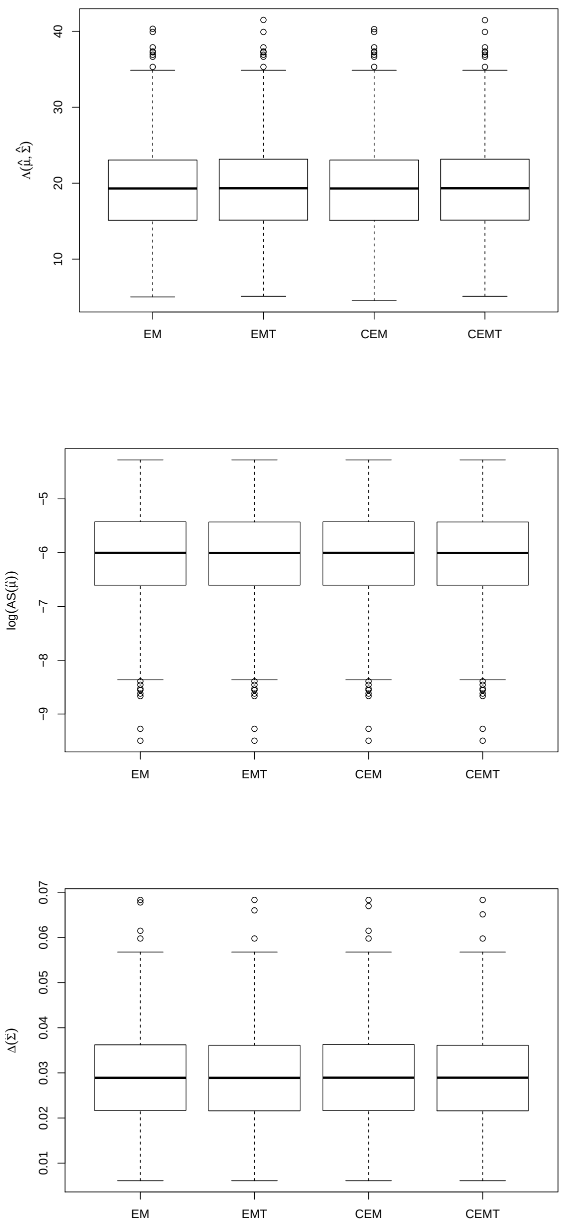


Figure SM–56: Performance of the estimators in the case $p = 5$, sample size $n = 500$, $\sigma = \pi/4$.

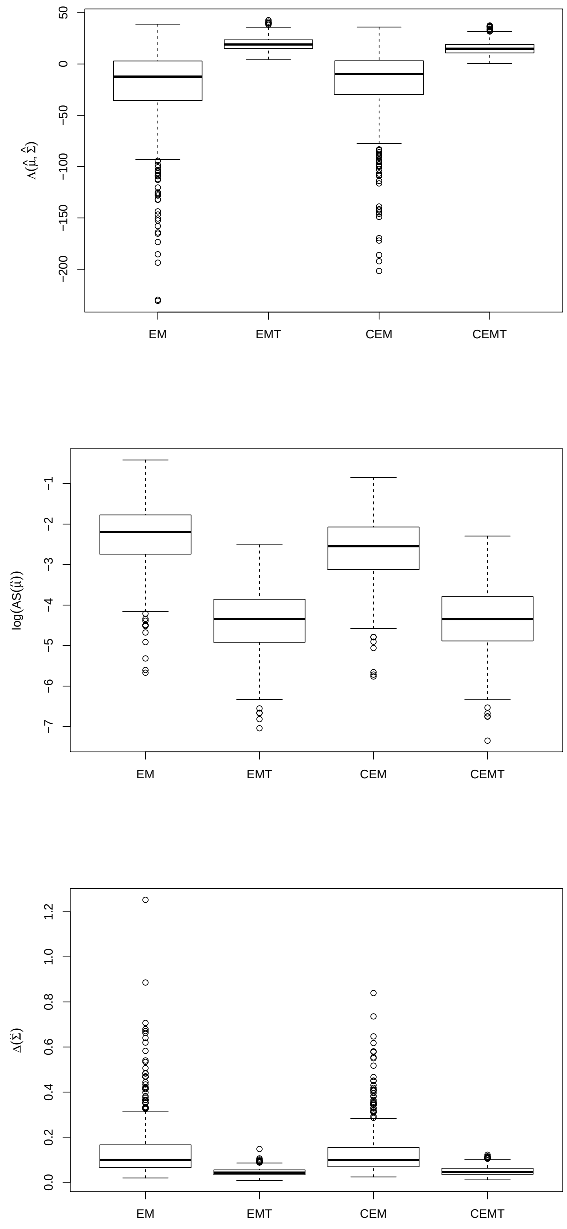


Figure SM–57: Performance of the estimators in the case $p = 5$, sample size $n = 500$, $\sigma = \pi/2$.

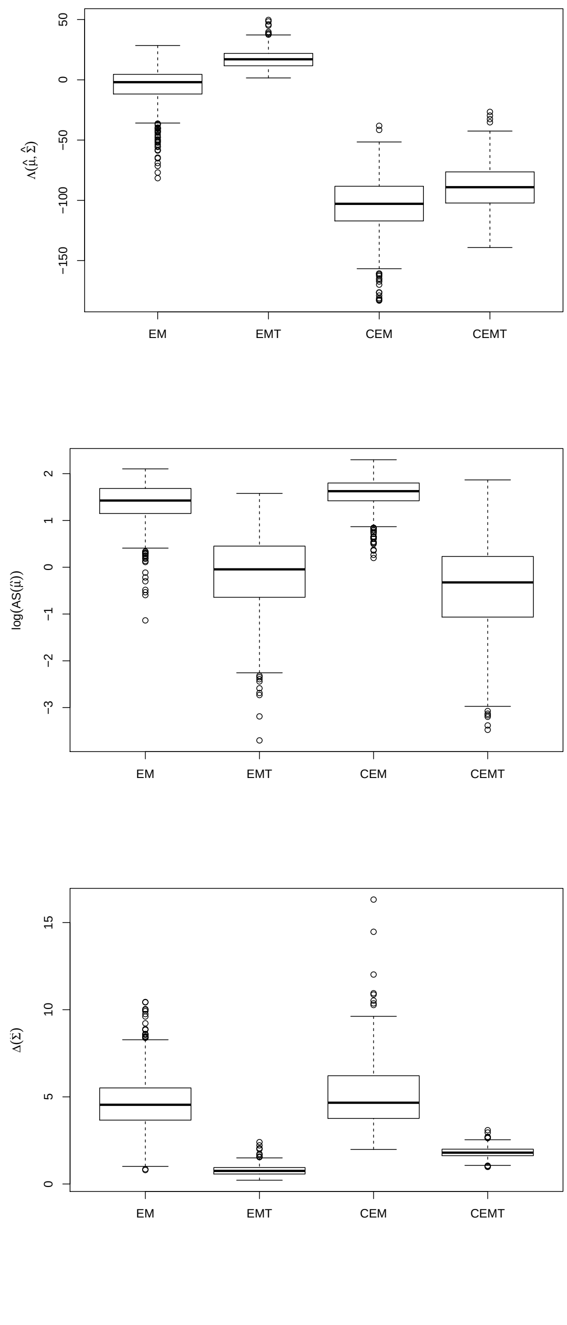


Figure SM–58: Performance of the estimators in the case $p = 5$, sample size $n = 500$, $\sigma = \pi$.

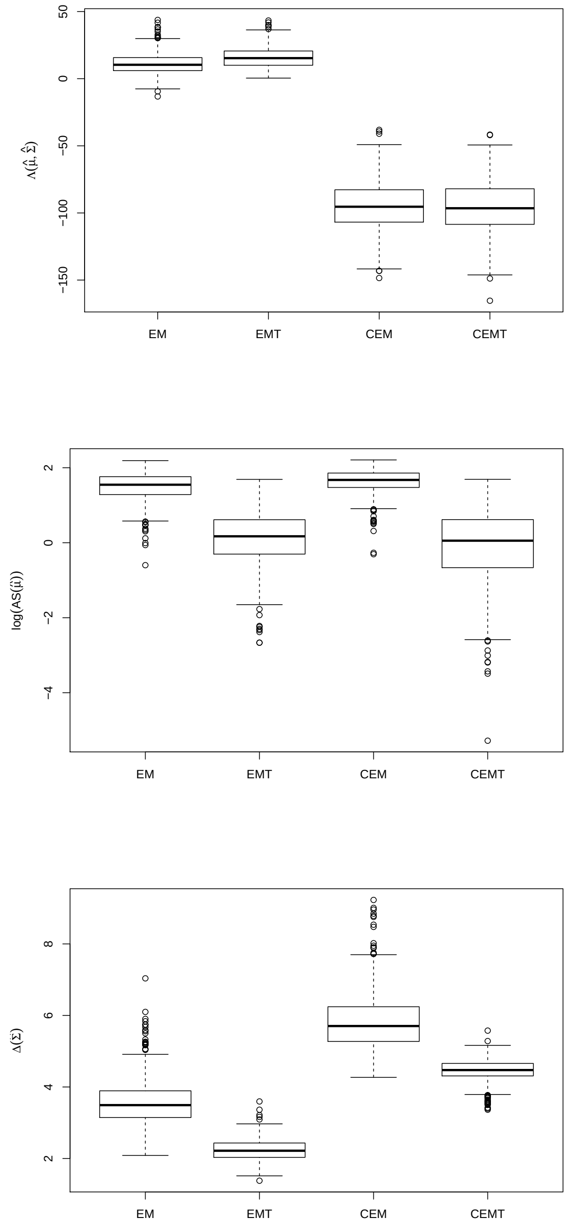


Figure SM–59: Performance of the estimators in the case $p = 5$, sample size $n = 500$, $\sigma = 3\pi/2$.

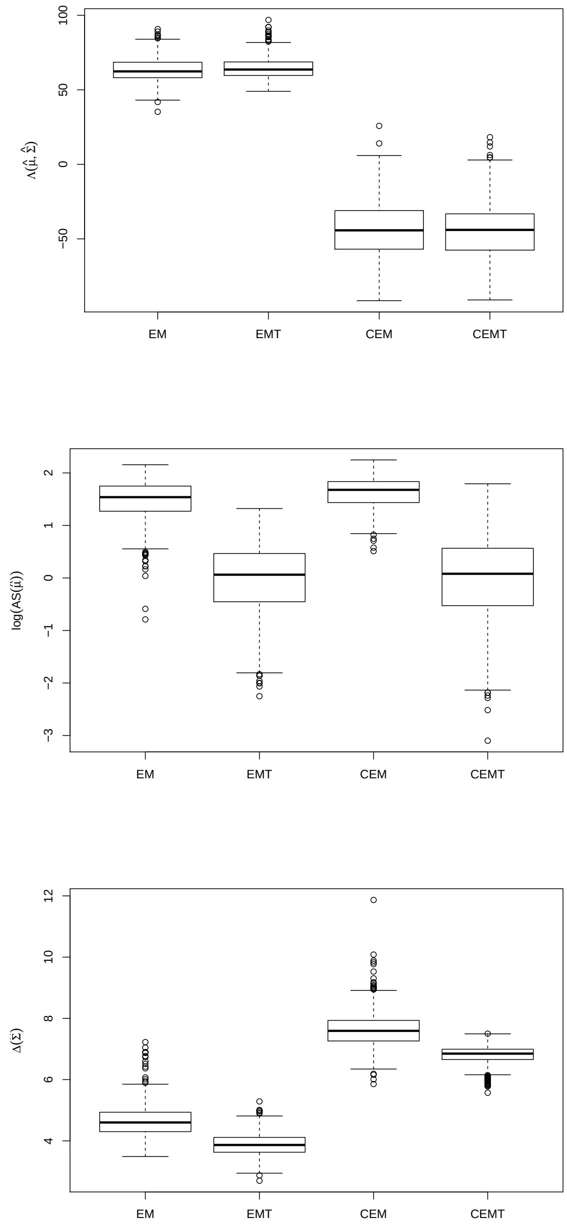


Figure SM–60: Performance of the estimators in the case $p = 5$, sample size $n = 500$, $\sigma = 2\pi$.

**SM–4.4** $p = 10$

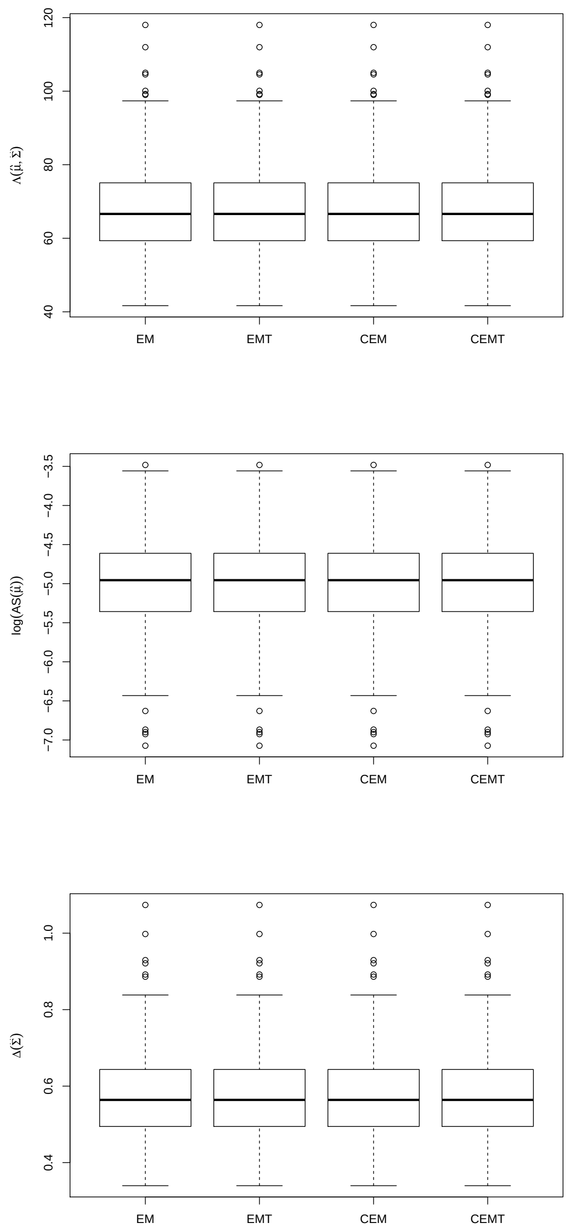


Figure SM–61: Performance of the estimators in the case $p = 10$, sample size $n = 100$, $\sigma = \pi/8$.

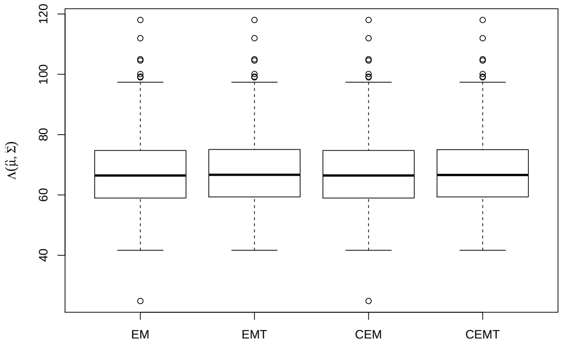


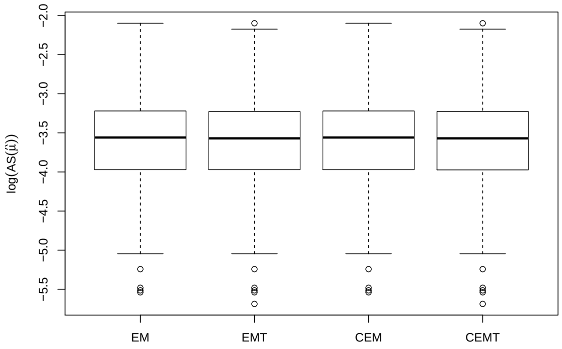


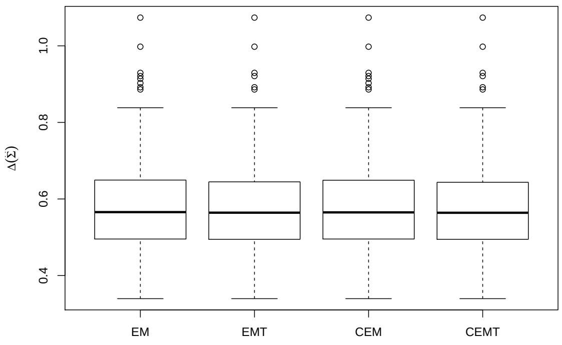


Figure SM–62: Performance of the estimators in the case $p = 10$, sample size $n = 100$, $\sigma = \pi/4$.

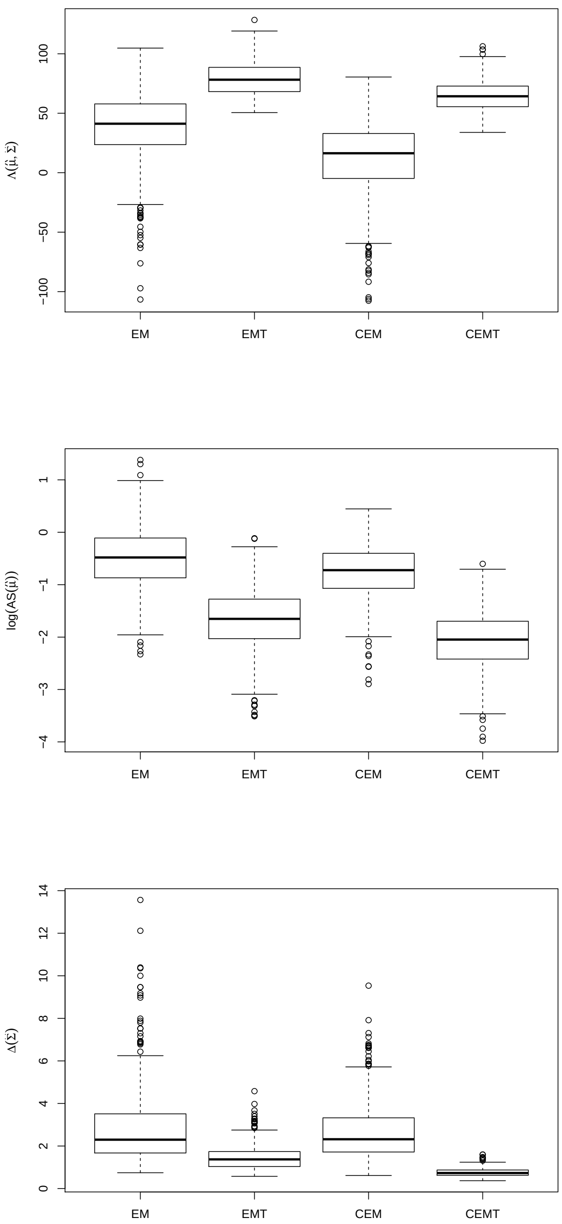


Figure SM–63: Performance of the estimators in the case $p = 10$, sample size $n = 100$, $\sigma = \pi/2$.

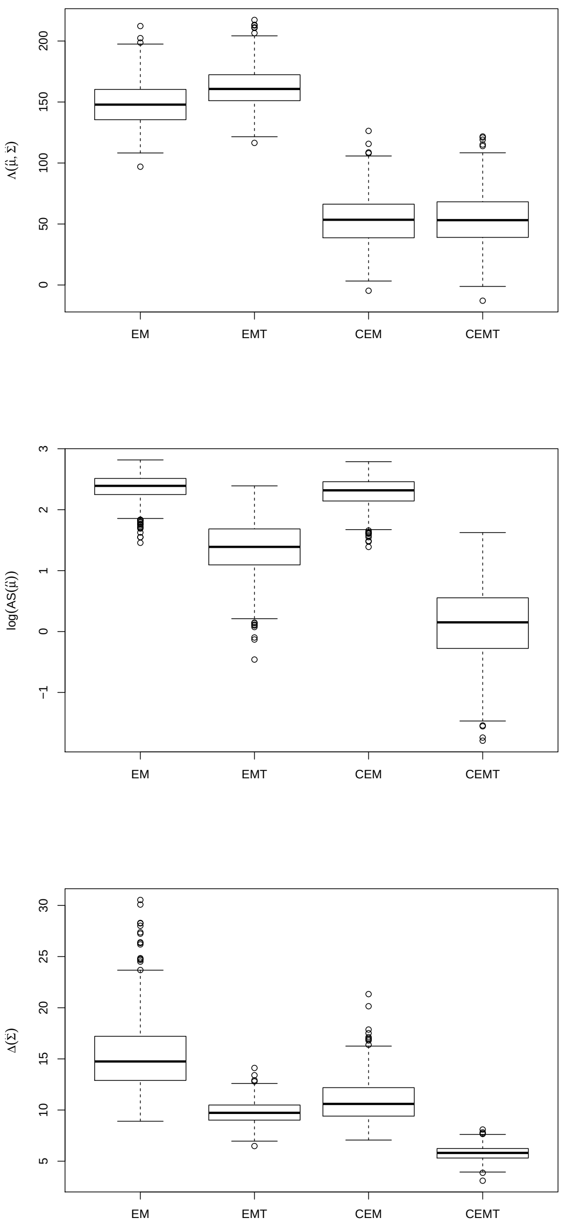


Figure SM–64: Performance of the estimators in the case $p = 10$, sample size $n = 100$, $\sigma = \pi$.

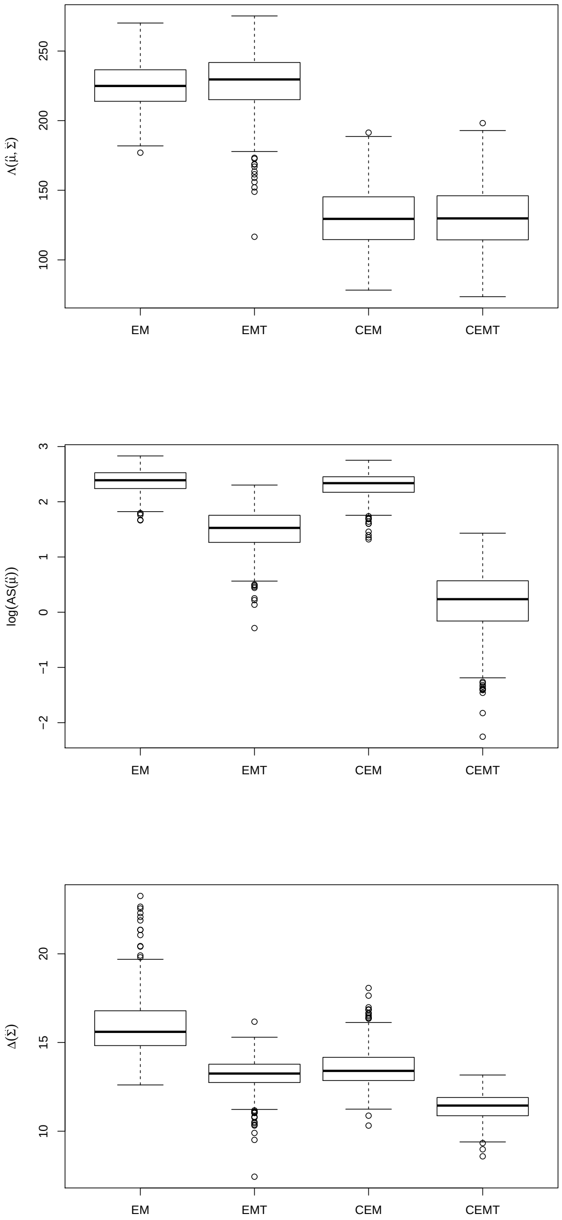


Figure SM–65: Performance of the estimators in the case $p = 10$, sample size $n = 100$, $\sigma = 3\pi/2$.

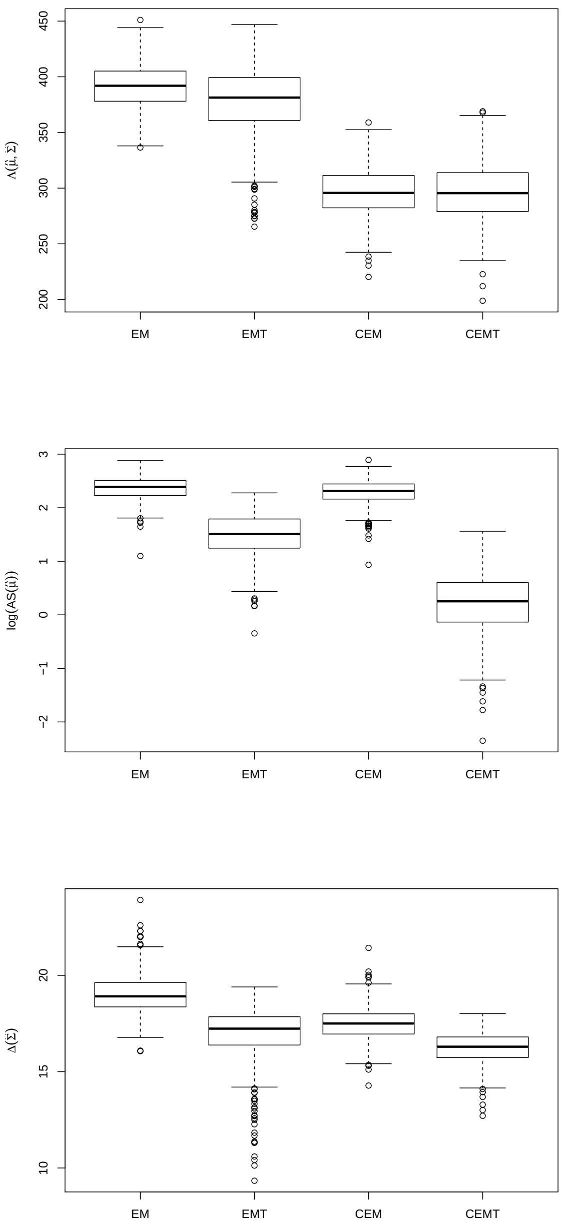


Figure SM–66: Performance of the estimators in the case $p = 10$, sample size $n = 100$, $\sigma = 2\pi$.

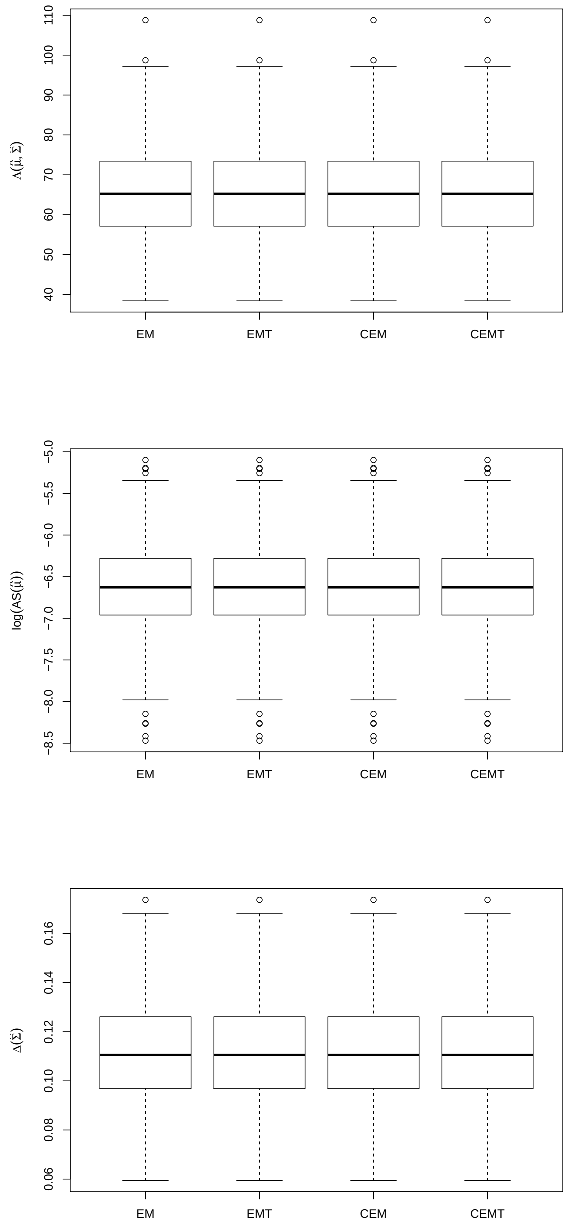


Figure SM–67: Performance of the estimators in the case $p = 10$, sample size $n = 500$, $\sigma = \pi/8$.

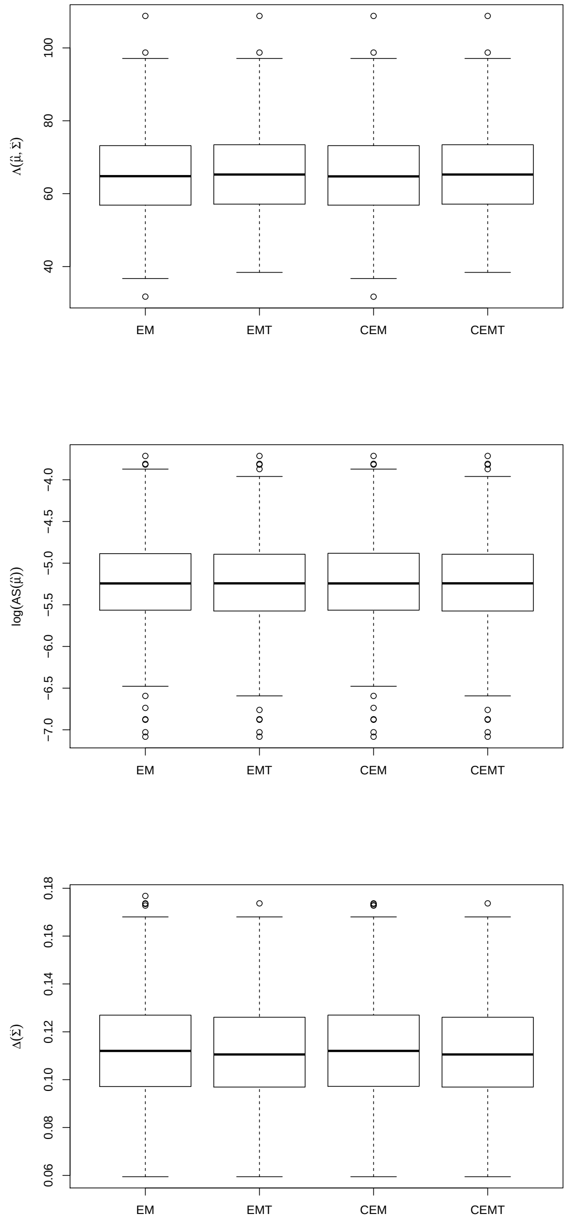


Figure SM–68: Performance of the estimators in the case $p = 10$, sample size $n = 500$, $\sigma = \pi/4$.

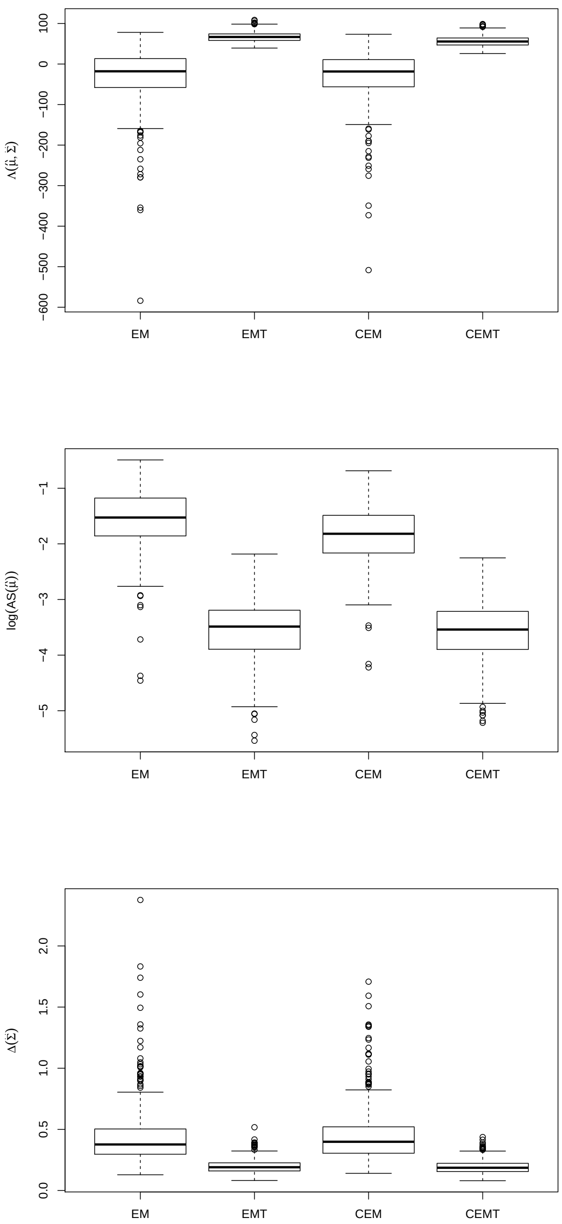


Figure SM–69: Performance of the estimators in the case $p = 10$, sample size $n = 500$, $\sigma = \pi/2$.

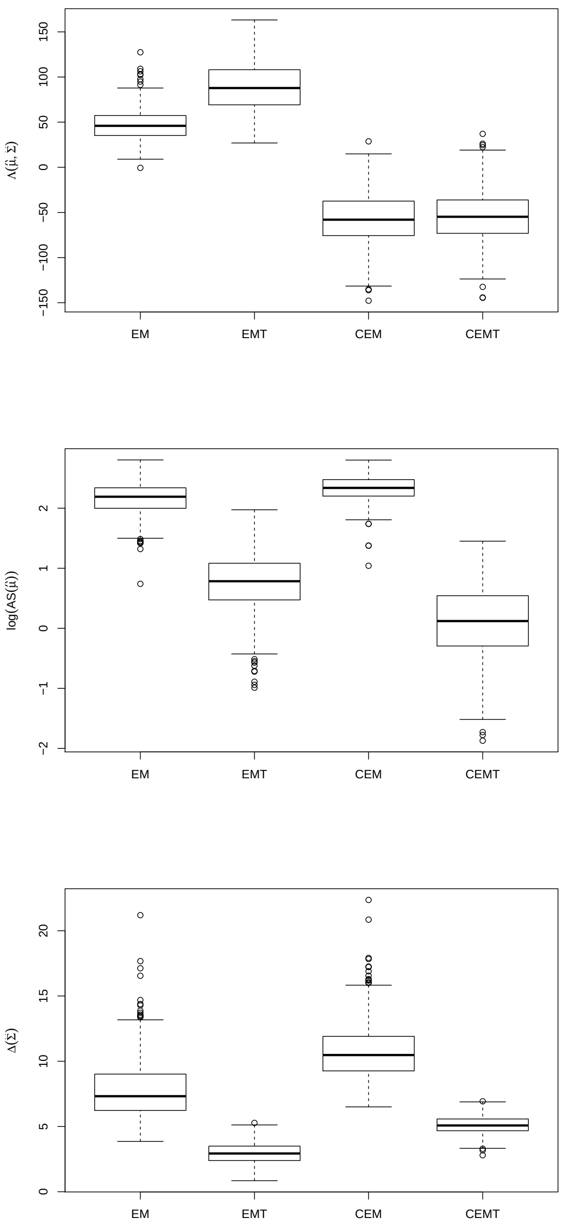


Figure SM–70: Performance of the estimators in the case $p = 10$, sample size $n = 500$, $\sigma = \pi$.

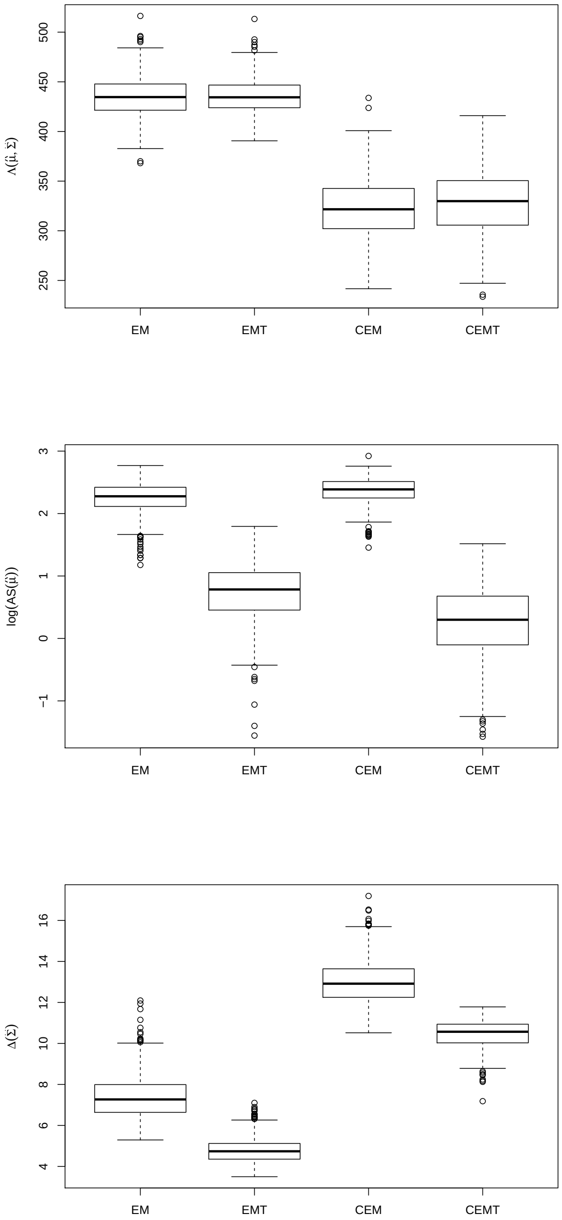


Figure SM–71: Performance of the estimators in the case $p = 10$, sample size $n = 500$, $\sigma = 3\pi/2$.

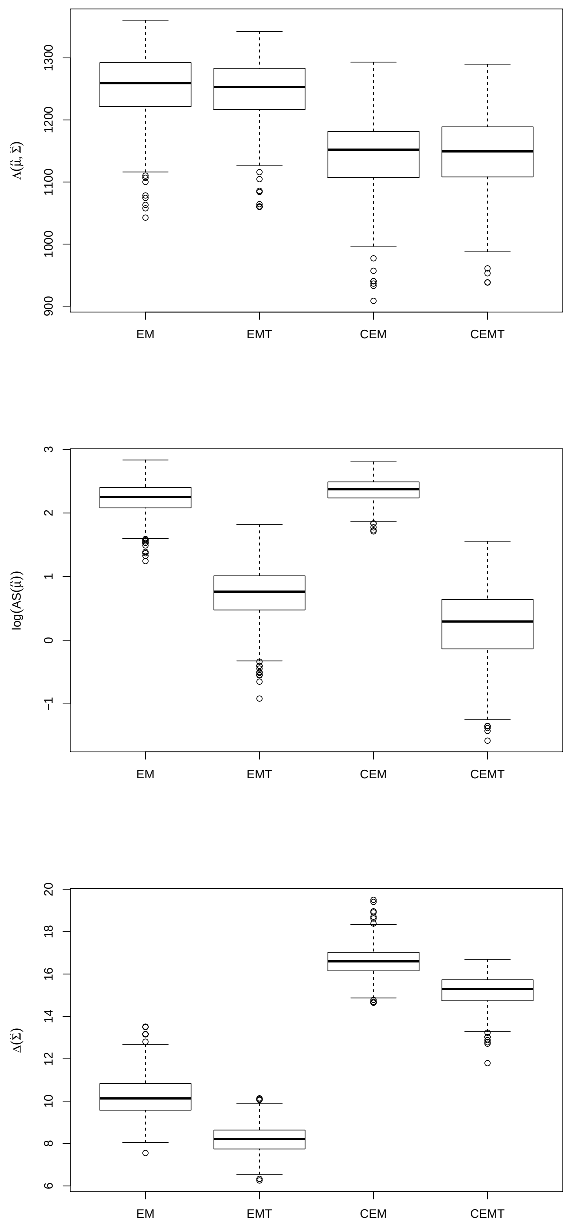


Figure SM–72: Performance of the estimators in the case $p = 10$, sample size $n = 500$, $\sigma = 2\pi$.
